# Supplementary material for: Unsupervised Point Cloud Pre-Training via Occlusion Completion
Source: arXiv:2010.01089 source file (2021-10-13)
Supplement: Supplementary file 2 [file appendix.tex]

\onecolumn
\todo{submit in a separate file}

% \begin{figure*}[t]
%     \centering
%     \vspace{-6ex}
%     \includegraphics[width=\linewidth]{resources/occulsion_completion.pdf}
%     \vspace{-3ex}
%     % \caption{\method\, is a self-supervised pre-training method composed of two steps: (a) occlusion $o(\cdot)$ of an input point cloud $\mathcal{P}$ based on a random camera view-point into a partial point cloud $\tilde{\mathcal{P}}$, and (b) a model $c(\cdot)$ that completes the occluded point cloud $\bar{\mathcal{P}}$ so that $\bar{\mathcal{P}} \approx \mathcal{P}$. We demonstrate that the completion model $c(\cdot)$ can be used as initialization for downstream tasks (e.g., classification, segmentation) leading to faster training and better generalization over existing methods.}
%     \caption{\abbrev  consists of two steps: (a) occlusion $o(\cdot)$ of a point cloud $\mathcal{P}$ based on a random camera view-point into a partial point cloud $\tilde{\mathcal{P}}$, and (b) a model $c(\cdot)$ that completes the occluded point cloud $\bar{\mathcal{P}}$ so that $\bar{\mathcal{P}} \approx \mathcal{P}$. We demonstrate that the completion model $c(\cdot)$ can be used as initialization for downstream tasks, leading to faster training and better generalization over existing methods.}
%     % \label{fig:overview}
%     \vspace{-3ex}
% \end{figure*}

\section{Design of the Completion Model}
Previous point completion models \citep{3D-EPN, yuan2018pcn,Tchapmi_2019_CVPR,WangAL20} all use an "encoder-decoder" architecture. The encoder maps a partial point cloud to a vector of a fixed dimension, and the decoder reconstructs the full point cloud. 

In the \abbrev experiments, we exclude the last few MLPs of PointNet and DGCNN, and use the remaining architecture as the encoder to map a partial point cloud into a 1024-dimensional vector. 
We adapt the folding-based decoder design from PCN, which is a two-stage point cloud generator that produces a coarse and a fine-grained output point cloud $(Y_{coarse}, Y_{fine})$ for each input. We removed all the batch normalisation layers in the folding-based decoder since we find it brings negative effects in the completion process in terms of Chamfer distance loss and convergent speed. On the basis of prior self-supervised learning methods, SimCLR~\citep{chen2020simple}, MoCo~\citep{he2019momentum} and BYOL~\citep{BYOL}, we find the batch normalisation is important in the encoder yet harmful for our decoder. Also, we find the L2 normalisation in the Adam optimiser is undesirable for completion training but brings improvements on the downstream fine-tuning tasks.

The predicted coarse point cloud $\hat{Y}_{coarse}$, which represents the global geometry of a shape, is generated via a set of fully connected layers. A folding-based generator is used to predict the local fine structures of each point in $\hat{Y}_{coarse}$, this results in $\hat{Y}_{fine}$. The folding based structures is proved to be good at approximating a smooth surface which reflects the local geometry. During training, $Y_{coarse}$ and $Y_{fine}$ are generated via randomly sampling 1024 and 16384 points from the mesh, respectively.

We use either Chamfer Distance (CD) or Earth Mover Distance (EMD) as the loss function for the completion model. We use a normalised and symmetric (thus commutative) version of Chamfer Distance (CD) to quantify the differences between two point clouds $\hat{P}$ and $P$:
\begin{gather}
    \mathrm{CD}(\hat{P}, P) = \frac{1}{|\hat{P}|}\sum_{\hat{x}\in \hat{P}}\min_{x\in P}||\hat{x}-x||_2 + \frac{1}{|P|}\sum_{x\in P}\min_{\hat{x}\in \hat{P}}||x-\hat{x}||_2.
\end{gather}
Note that it is no need that the two point cloud $\hat{P}$ and $P$ have the same size. But when calculating the Earth Mover Distance (EMD), $\hat{P}$ and $P$ are usually required to have the same number of points:
\begin{gather}
    \mathrm{EMD}(\hat{P}, P) = \min_{\phi:\hat{P}\rightarrow P}\frac{1}{|\hat{P}|}\sum_{\hat{x}\in \hat{P}}||\hat{x}-\phi(\hat{x})||_2,
\end{gather}
where $\phi$ is a bijection between points in $\hat{P}$ and $P$. Note that EMD is not commutative. Since finding the optimal mapping $\phi$ is quite time consuming, we use its approximation form~\cite{bertsekas1985distributed}.

The loss $l$ of the completion task is a adaptive weighted sum of coarse and fine generations:
\begin{gather}
    l = d_1(\hat{Y}_{coarse}, Y_{coarse}) + \alpha * d_2(\hat{Y}_{fine}, Y_{fine}),
\end{gather}
where the step-wise trade-off coefficient $\alpha$ incrementally grows during training. In our experiments, we find that even with approximation, it is still suboptimal to use EMD for $d_2$, since it is inefficient to solve the approximate bijection mapping $\phi$ for over 16k point pairs. We evaluate both `EMD+CD' and `CD+CD' combinations for the loss $l$. 
% As shown in Table.~\ref{table:emd-cd}, 
% During exploration on the OcCo pre-training settings, 
We have found that \abbrev with `EMD+CD' loss has achieved comparable performance yet longer time in the downstream classification tasks compared with the `CD+CD'. We use `CD+CD' as the loss function in the \abbrev pre-training process described in Section.~\ref{sec:pretrain_settings} in terms of simplicity and efficiency.

\section{Qualitative Results from Completion Pre-Training}
In this section, we show some qualitative results of \abbrev pre-training by visualising the input, coarse output, fine output and ground truth at different training epochs and encoders. In Figure.~\ref{fig:qualitative_occo_pcn}, Figure.~\ref{fig:qualitative_occo_pointnet} and Figure.~\ref{fig:qualitative_occo_dgcnn}, we notice that the trained completion models are able to complete even difficult occluded shapes such as plants and planes.
In Figure.~\ref{fig:failuare_occo} we plot some failure examples of completed shapes, possibly due to their complicated fine structures, while it is worth mentioning that the completed model can still completed these objects under the same category.

% \section{Qualitative Results in applying OcCo Models to Complete Real Data}

\section{Visualisation of part activation map and ground truth}
\label{sec:learned_feat}
\begin{figure}[H]
    \centering
     \includegraphics[width=.95\textwidth]{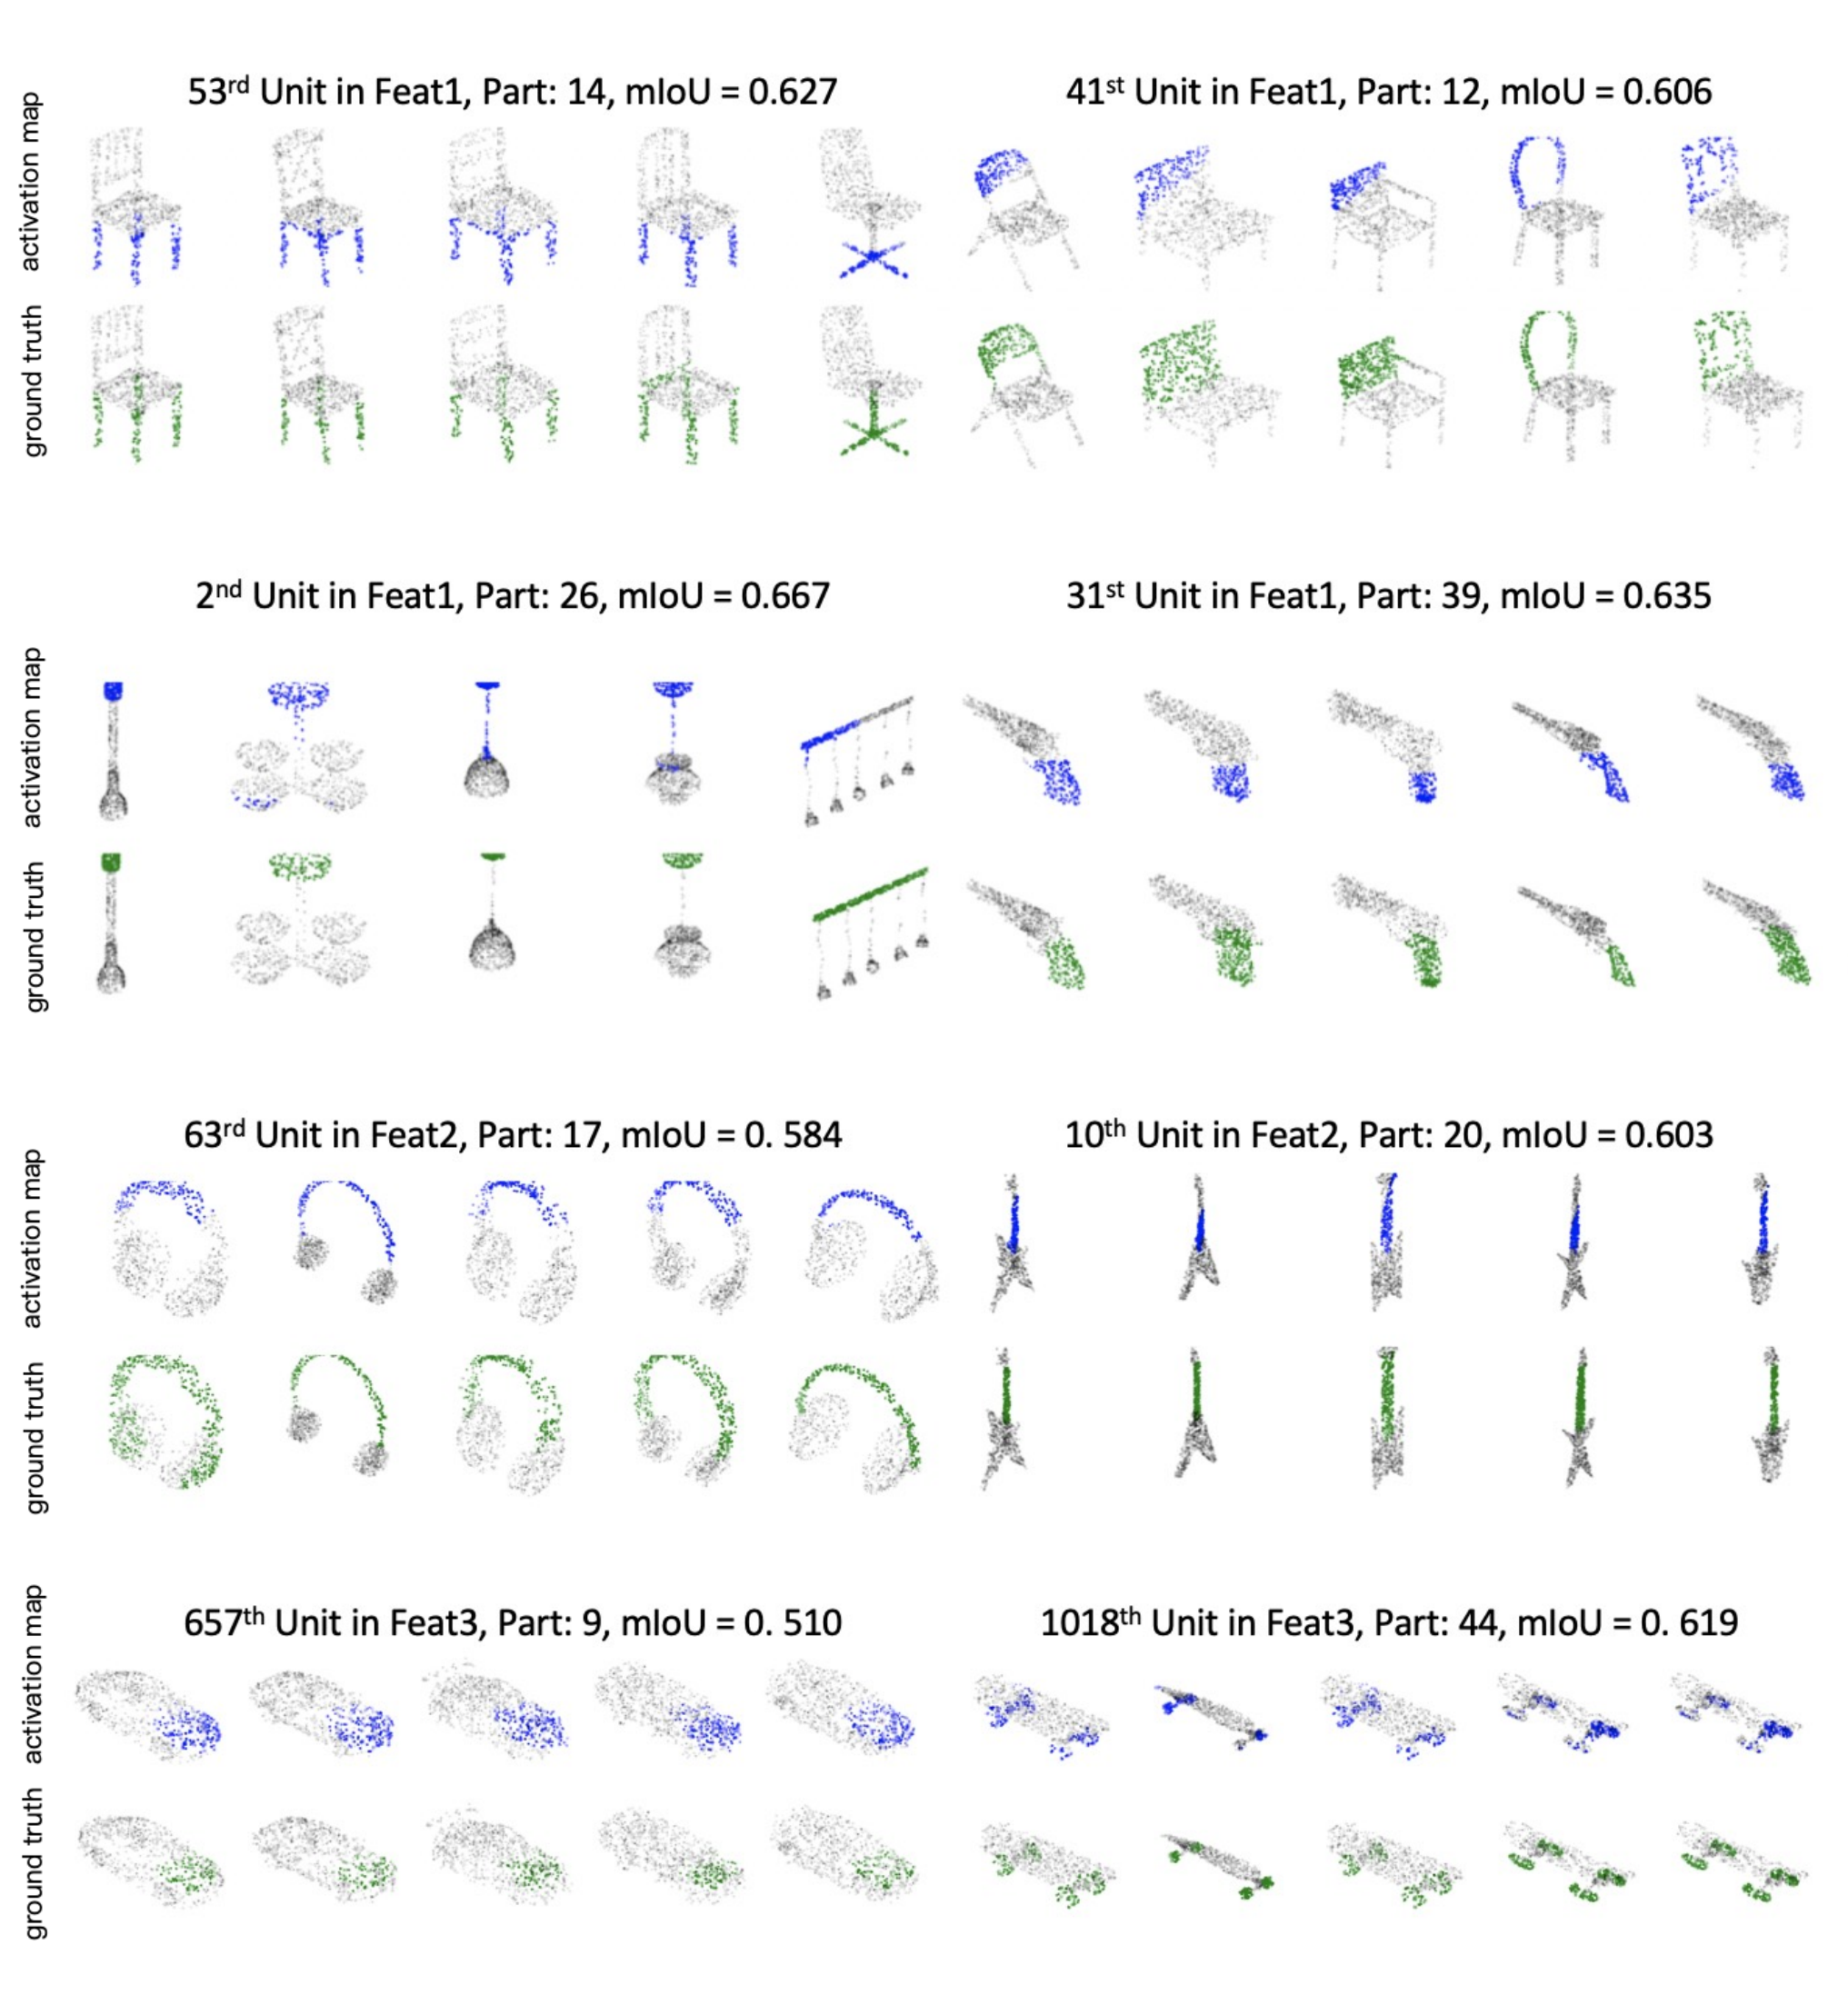}
     \vspace{-3ex}
     \caption{Learned features in OcCo pre-training}
     \label{fig:learned_feat}
\end{figure}

\section{Analysis on the Effects of OcCo Pre-Training Datasets}
We compare the occluded datasets based on ModelNet40 and ShapeNet8 for the \abbrev pre-training. We construct the ModelNet Occluded using the methods described in Section~\ref{sec:method} and for ShapeNet Occluded we directly use the data provided in the PCN, whose generation method are similar but not exactly the same with ours. Basic statistics of these two datasets are reported in Table~\ref{tab:occo_stats}. 
% Note that both datasets use the same method to generate occluded point cloud objects.
Compared with the ShapeNet Occluded dataset which is publicized by PCN and used in all the follow-ups\citep{Tchapmi_2019_CVPR,WangAL20}, our occluded ModelNet dataset has more object categories, more view-points, more points per object and therefore is more challenging. We believe such differences will help the encoder models learn a more comprehensive and robust representation which is transferable to downstream tasks. To support our idea, we perform \abbrev pre-training on these two datasets respectively, and test their performance on ModelNet40 and ShapeNet Occluded classification benchmarks. 
\begin{table}[H]
\small
\centering
\vspace{-2ex}
\caption{Statistics of occluded datasets for \abbrev pre-training}
\begin{tabular}{c|c|c|c|c}
\bottomrule
Name & \# of Class & \# of Object & \# of Views & \# of Points/Object \\ \hline
ShapeNet Occluded (PCN) & 8  & 30974 & 8  & 1045      \\ \hline
ModelNet Occluded (\abbrev)   & 40 & 12304 & 10 & 20085    \\ \toprule
% ModelNet40 Middle & 40 & 12304 & 10 &        \\ \hline
% ModelNet40 Coarse & 40 & 12304 & 10 &        \\ \hline
\end{tabular}
\label{tab:occo_stats}
\vspace{-3ex}
\end{table}
The reason of choosing these two datasets for benchmarking is, ShapeNet Occluded is the out-of-domain data for the models pre-trained on ModelNet Occluded, and vice versa. We believe it will give us sufficient information on which occluded dataset should be preferred the \abbrev pre-training. 
The Results are shown in Table~\ref{table:occo-dataset}.
\begin{table}[H]
\centering
% \vspace{-2ex}
\caption{Performance of \abbrev pre-trained models with different pre-trained datasets}
\begin{tabular}{c|c|c|c}\bottomrule
\multicolumn{2}{c|}{\abbrev Settings} & \multicolumn{2}{c}{Classification Accuracy} \\\toprule\bottomrule
Encoder & Pre-Trained Dataset & ModelNet Oc & ShapeNet Oc \\\hline
\multirow{2}{*}{PointNet} & ShapeNet Oc & 81.0 & 94.1 \\\cline{2-4}
 & ModelNet Oc & \textbf{85.6} & \textbf{95.0} \\\hline
\multirow{2}{*}{PCN} & ShapeNet Oc & 81.6 & 94.4 \\\cline{2-4}
 & ModelNet Oc & \textbf{85.1} & \textbf{95.1} \\\hline
 \multirow{2}{*}{DGCNN} & ShapeNet Oc & 86.7 & 94.5 \\\cline{2-4}
 & ModelNet Oc & \textbf{89.1} & \textbf{95.1} \\\toprule
\end{tabular}
\vspace{-3ex}
\label{table:occo-dataset}
\end{table}

From Table~\ref{table:occo-dataset}, we see that the \abbrev models pre-trained on ShapeNet Occluded do not perform as well as the ones pre-trained on ModelNet Occluded in most cases. Thus in our experiments, we reports the results pre-trained on ModelNet Occluded.

By visualising the objects from the ShapeNet Occluded (in Figure.~\ref{fig:shapenet_failure}), we believe this performance deficiency in downstream fine-training of pre-trained models is due to the quality of the generated occluded point clouds (in comparison with our generated dataset shown in Figure.~\ref{fig:dataoverview}). Further, we think our dataset is a more challenging task for all the present completion models.

\begin{figure}[H]
    \centering
     \includegraphics[width=\textwidth]{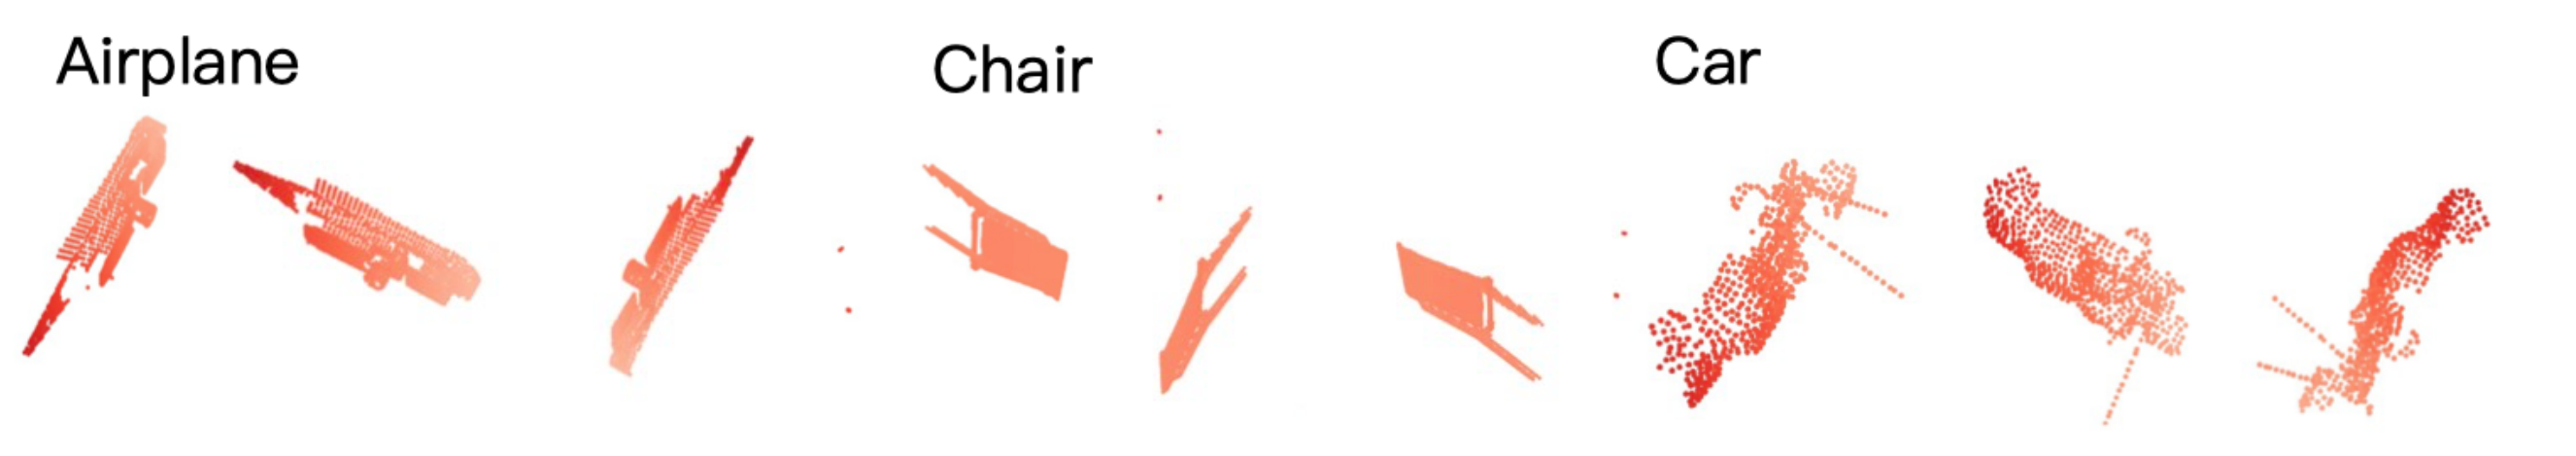}
     \caption{Examples from ShapeNet Occluded which fail to depict the underlying object shapes}
     \label{fig:shapenet_failure}
\end{figure}

\section{Detailed Results on training a Linear SVM for Classification}
We first described the benchmark datasets that are used for classification in Table~\ref{tab:cls_data}.

To make a comprehensive and convincing comparison, we follow the similar procedures from \citep{achlioptas2017learning,han2019view,sauder2019self,wu2016learning,yang2018foldingnet}, to train a linear Support Vector Machine (SVM) to examine the generalisation of \abbrev encoders that are pre-trained on occluded objects from ModelNet40. For all six classification datasets, we fit a linear SVM on the output 1024-dimensional embeddings of the train split and evaluate it on the test split. Since \citet{sauder2019self} have already proven their methods are better than the prior, here we only systematically compare with theirs. We report the results\footnote{In our implementation, we also provide an alternative to use grid search to find the optimal set of parameters for SVM with a Radial Basis Function (RBF) kernel. In this setting, all the \abbrev pre-trained models have outperformed the random initialised and Jigsaw pre-trained ones by a large margin as well.} in Table~\ref{tab:svm-classification}, we can see that all \abbrev models achieve superior results compared to the randomly-initialized counterparts, demonstrating that \abbrev pre-training helps the generalisation both in-domain and cross-domain. 
\begin{table}[H]
\centering
\vspace{-2ex}
\small
\caption{linear SVM on the output embeddings from random, Jigsaw and OcCo initialised encoders}
\begin{tabular}{c|c|c|c|c|c|c|c|c|c}
\bottomrule \multirow{2}{*}{Dataset} & 
\multicolumn{3}{c|}{PointNet} & \multicolumn{3}{c|}{PCN} & \multicolumn{3}{c}{DGCNN} \\ \cline{2-10}
 & Rand & Jigsaw & \abbrev& Rand & Jigsaw & \abbrev & Rand & Jigsaw & \abbrev \\ \toprule \bottomrule
ShapeNet10   & 91.3 & 91.1 & \textcolor{blue}{93.9} & 88.5 & 91.8 & \textbf{94.6} & 90.6 & 91.5 & \textcolor{blue}{94.5} \\\hline
ModelNet40   & 70.6 & 87.5 & \textcolor{blue}{88.7} & 60.9 & 73.1 & \textcolor{blue}{88.0} & 66.0 & 84.9 & \textbf{89.2} \\\hline
ShapeNet Oc  & 79.1 & 86.1 & \textcolor{blue}91.1 & 72.0 & 87.9 & \textcolor{blue}90.5 & 78.3 & 87.8 & \textbf{91.6} \\\hline
ModelNet Oc  & 65.2 & 70.3 & \textcolor{blue}{80.2} & 55.3 & 65.6 & \textbf{83.3} & 60.3 & 72.8 & \textcolor{blue}{82.2} \\\hline
ScanNet10    & 64.8 & 64.1 & \textcolor{blue}{67.7} & 62.3 & 66.3 & \textbf{75.5} & 61.2 & 69.4 & \textcolor{blue}{71.2} \\\hline
ScanObjectNN & 45.9 & 55.2 & \textcolor{blue}69.5 & 39.9 & 49.7 & \textcolor{blue}{72.3} & 43.2 & 59.5 & \textbf{78.3} \\\toprule
\end{tabular}
\label{tab:svm-classification}
\vspace{-4ex}
\end{table}

% \section{T-SNE}
% In Figure~\ref{fig:tsne}, we use t-SNE \citep{tsne} to visualise the embeddings of \abbrev models on ShapeNet10. We can see that the separable clusters are formed for different object classes.
% \begin{figure}[H]
%     \centering
%      \includegraphics[width=\textwidth]{resources/tsne_small.pdf}
%      \vspace{-3ex}
%      \caption{T-SNE visualisation of the learned embeddings of ShapeNet objects from OcCo pre-trained encoders, all the three encoders are pre-trained on occluded objects from ModelNet40.}
% \end{figure}

% \section{Completed Real World Occluded Objects}
% ScanObjectNN and ShapeNet Oc\\
% Story: why OcCo brings larger improvements in classifying partial point cloud objects. 

\section{Re-Implementation Details of "Jigsaw" Pre-Training Methods}
In this section, we describe how we reproduce the 'Jigsaw' pre-training methods from \citep{sauder2019self}. Following their description, we first separate the objects/chopped indoor scenes into $3^3=27$ small cubes and assign each point a label indicting which small cube it belongs to. We then shuffle all the small cubes, and train a model to make a prediction for each point. We reformulate this task as a 27-class semantic segmentation, for the details on the data generation and model training, please refer to our released code.
% : \href{https://github.com/hansen7/OcCo}{{\color{blue}https://github.com/hansen7/OcCo}}

\section{More comparisons}
In Table~\ref{tab:classification_benchmark}, we compare \abbrev with prior point-cloud-specific pre-training methods \citep{alliegro2020joint}.
% \footnote{As the authors did not respond to code requests, we compare to their published results using the same setup.}  
Our method obtains the best results on all settings. 
These results confirm that the inductive bias learned by reconstructing occluded point clouds is stronger than one based in reconstructing permuted clouds \citep{alliegro2020joint,sauder2019self}. Specifically, we believe that because \abbrev does not rearrange object parts but instead creates point clouds that resemble real-world 3D sensor occlusions, the initialization better encodes realistic object shape and context.

\begin{table}[H]
\centering
\vspace{-1ex}
\caption{Accuracy comparison between OcCo and prior pre-training baselines \cite{alliegro2020joint} on 3D object recognition benchmarks. ModelNet40-20\% means only 20\% of training data are used.}
\begin{tabular}{c|c|c|c|c}
\bottomrule Baseline & Dataset & Rand & \citet{alliegro2020joint} & \abbrev \\ 
\toprule \bottomrule
\multirow{3}{*}{PointNet} & {ModelNet40} & 89.2 & 89.7 & \textbf{90.2} \\\cline{2-5}
 & {ModelNet40-20\%} & 82.9 & 83.1 & \textbf{83.6} \\\cline{2-5}
 & {ScanObjectNN (OBJ\_BG)} & 73.7 & 71.3 & \textbf{80.2} \\\hline
\toprule
\end{tabular}
\label{tab:classification_benchmark}
\end{table}

\section{Labelled Sample Efficiency \label{sec:efficiency}}

We investigate whether \abbrev pre-training can improve the labelled sample efficiency of downstream tasks. Specifically, we reduce the labelled samples to 1\%, 5\%, 10\% and 20\% of the original training set for the ModelNet40 object classification task, and evaluate on the full test set. 

% \subsection{Learning Curves}
% \label{subsec:train_convergence}

As shown in Table \ref{tab:few_shot}, OcCo-initialized models achieve superior results compared to the randomly-initialized models, demonstrating that \abbrev with in-domain pre-training improves labelled sample efficiency. 

\begin{table}
\centering
\caption{Sample efficiency with randomly-initialized and OcCo-initialized models.} %\abbrev initialization uses models pre-trained on the occluded dataset from ModelNet40.}
\begin{tabular}{c|c|c|c|c|c|c|c|c|c}
\bottomrule \multirow{2}{*}{Baseline} & 
\multicolumn{3}{c|}{PointNet} & \multicolumn{3}{c|}{PCN} & \multicolumn{3}{c}{DGCNN} \\ \cline{2-10}
 & Rand & Jigsaw & \abbrev& Rand & Jigsaw & \abbrev & Rand & Jigsaw & \abbrev \\ \toprule \bottomrule
1\%  & 56.9 & 55.7 & \textcolor{blue}{58.1} & 57.8 & 59.6 & \textcolor{blue}{60.4} & 60.0 & 59.9 & \textbf{60.5} \\\hline
5\%  & 73.9 & 74.3 & \textcolor{blue}{74.9} & 73.2 & 75.8 & \textcolor{blue}{76.7} & 79.4 & 79.2 & \textbf{79.7} \\\hline
10\% & 80.6 & \textcolor{blue}{81.3} & 81.1 & 81.1 & 82.1 & \textcolor{blue}{82.6} & 84.4 & 84.4 & \textbf{84.5} \\\hline
20\% & 83.6 & \textcolor{blue}{84.2} & \textcolor{blue}{84.2} & 83.6 & 84.2 & \textcolor{blue}{84.4} & 86.5 & 86.7 & \textbf{87.2} \\ %\hline %\hline
%100\% &  89.2 & 90.2 & 89.6 & 90.5 & 92.2 & \textbf{93.1}
%\\
\toprule
\end{tabular}
\vspace{-3ex}
% \label{tab:few_shot}
\end{table}

\section{Semantic Segmentation on Urban Scale Scans}

\begin{figure}[t]
    % \vspace{-7ex}
    \centering
     \includegraphics[width=\textwidth]{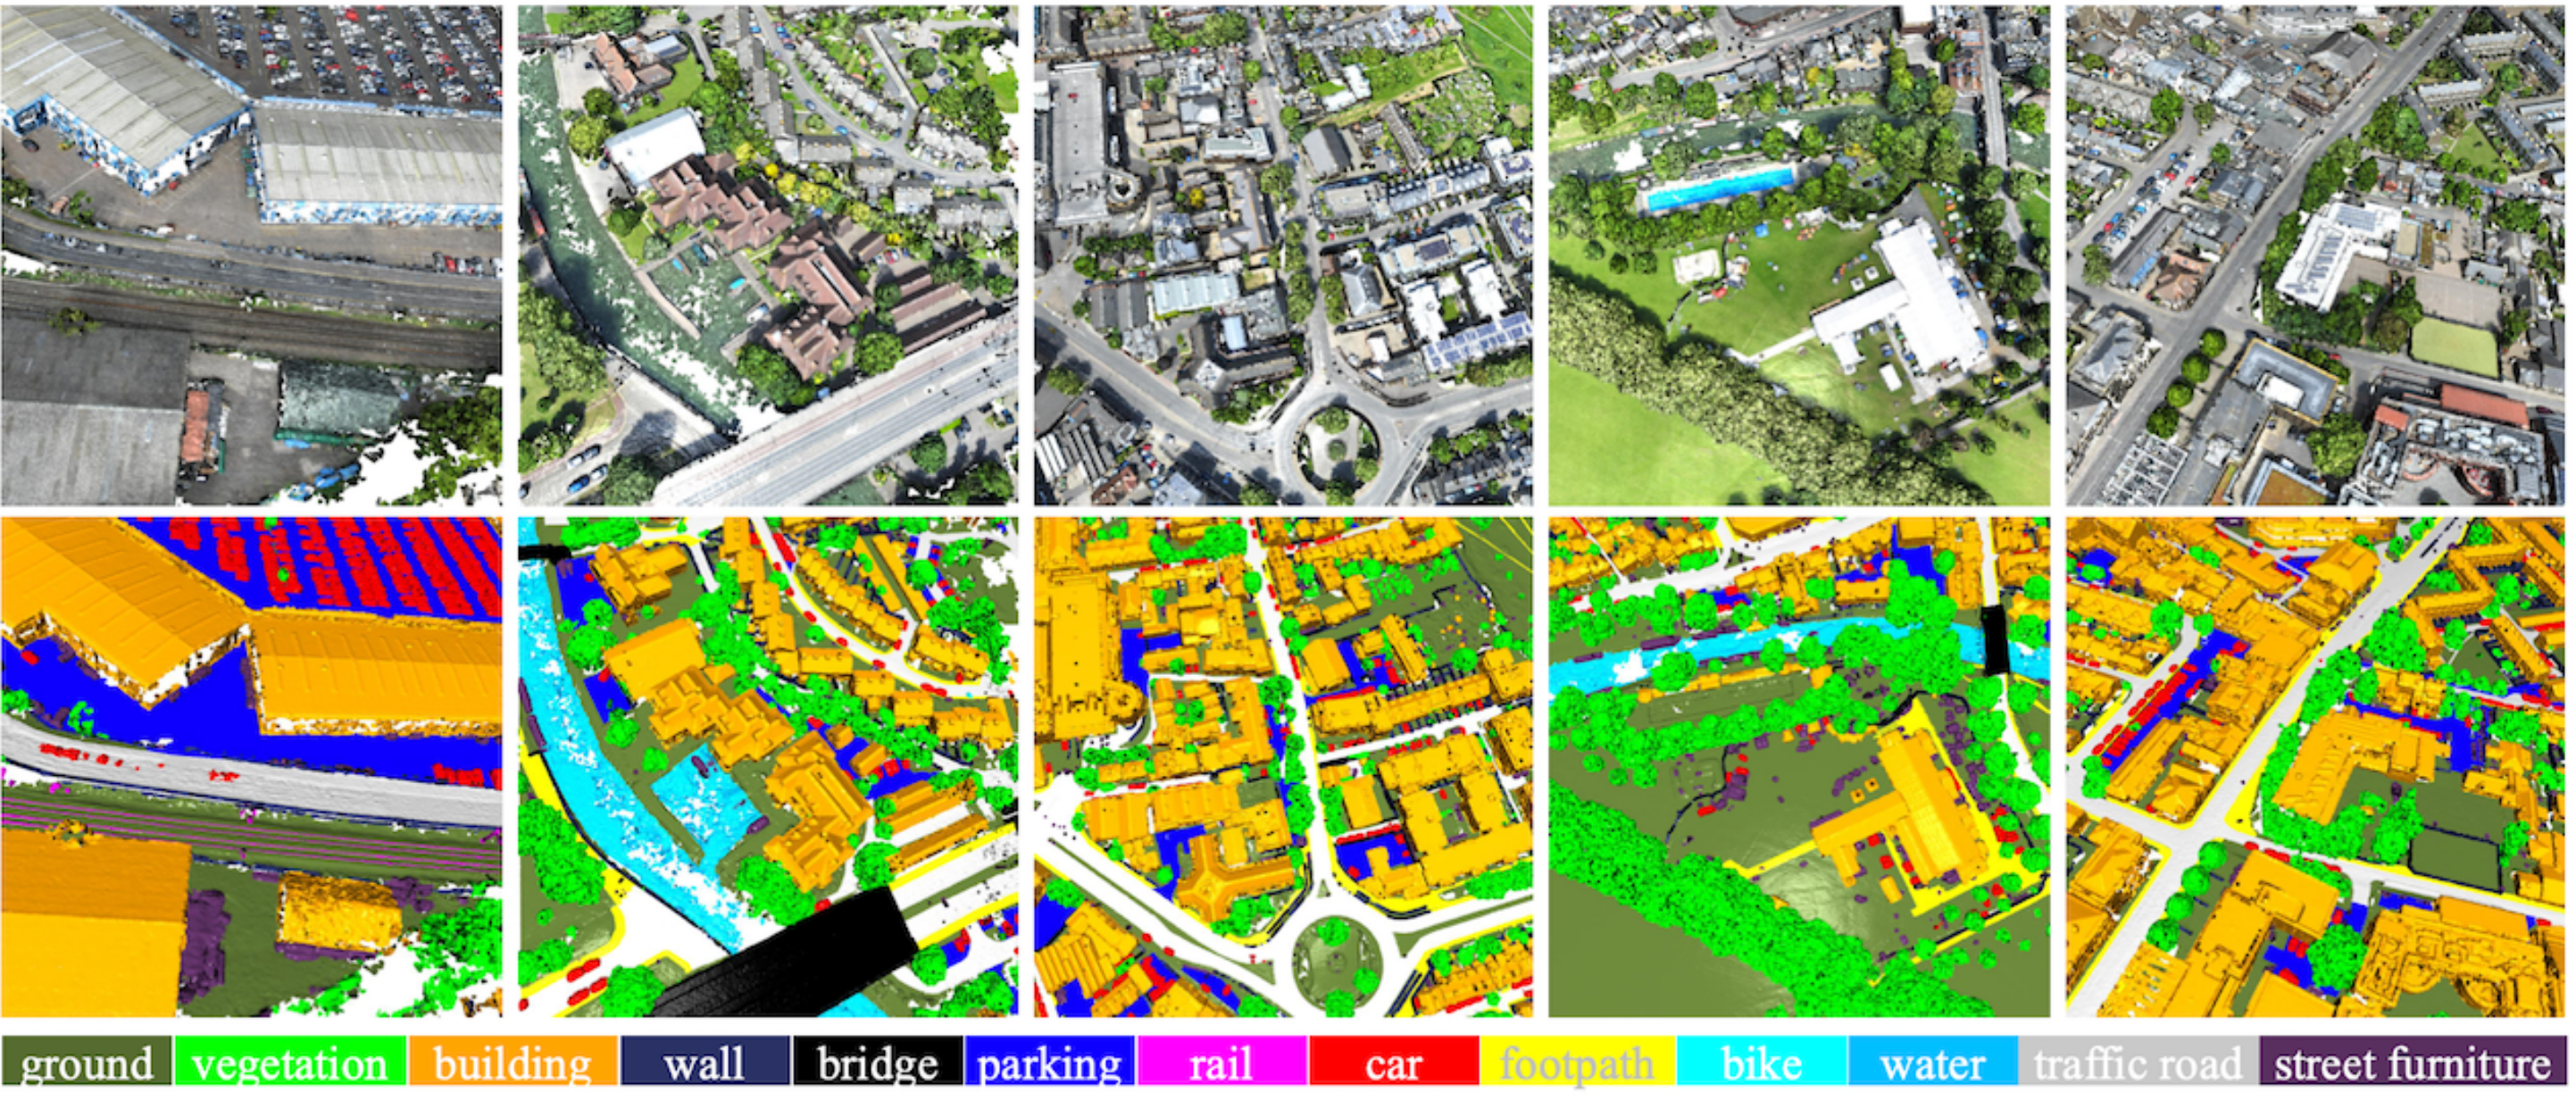}
     \vspace{-3ex}
     \caption{Overview of SensetUrban dataset, from~\cite{hu2020towards}}
     \vspace{-1ex}
\end{figure}

\begin{table}[t]\small
\setlength{\tabcolsep}{3pt}
\centering
\caption{Semantic segmentation results on SensatUrban.}
\begin{tabular}{ccccccccccccccccc}\bottomrule 
& \rotatebox{90}{OA(\%)} & \rotatebox{90}{mAcc(\%)} & \rotatebox{90}{mIoU(\%)\,\,} & \rotatebox{90}{ground} & \rotatebox{90}{veg} & \rotatebox{90}{building} & \rotatebox{90}{wall} & \rotatebox{90}{bridge} & \rotatebox{90}{parking} & \rotatebox{90}{rail} & \rotatebox{90}{traffic} & \rotatebox{90}{street} & \rotatebox{90}{car} & \rotatebox{90}{footpath} & \rotatebox{90}{bike} & \rotatebox{90}{water} \\\toprule
PointNet & 86.29 & 53.33 & 45.10 & 80.05 & 93.98 & 87.05 & 23.05 & 19.52 & 41.80 & 3.38 & 43.47 & 24.20 & 63.43 & 26.86 & 0.00 & 79.53 \\ 
% PointNet-Jigsaw & 87.38 & 56.97 & 47.90 & 83.36 & 94.72 & 88.48 & 22.87 & 30.19 & 47.43 & 15.62 & 44.49 & 22.91 & 64.14 & 30.33 & 0.00 & 77.88 \\ 
PointNet-OcCo & 87.87 & 56.14 & 48.50 & 83.76 & 94.81 & 89.24 & 23.29 & 33.38 & 48.04 & 15.84 & 45.38 & 24.99 & 65.00 & 27.13 & 0.00 & 79.58 \\\toprule\bottomrule
PCN & 86.79 & 57.66 & 47.91 & 82.61 & 94.82 & 89.04 & 26.66 & 21.96 & 34.96 & 28.39 & 43.32 & 27.13 & 62.97 & 30.87 & 0.00 & 80.06 \\
PCN-OcCo & 87.32 & 57.01 & 48.44 & 83.20 & 94.79 & 89.25 & 25.89 & 19.69 & 40.90 & 28.52 & 43.46 & 24.78 & 63.08 & 31.74 & 0.00 & 84.42 \\\toprule\bottomrule
DGCNN  & 87.54 & 60.27 & 51.96 & 83.12 & 95.43 & 89.58 & 31.84 & 35.49 & 45.11 & 38.57 & 45.66 & 32.97 & 64.88 & 30.48 & 0.00 & 82.34 \\
DGCNN-OcCo & 88.67 & 61.35 & 53.31 & 83.64 & 95.75 & 89.96 & 29.22 & 41.47 & 46.89 & 40.64 & 49.72 & 33.57 & 70.11 & 32.35 & 0.00 & 79.74 \\ \toprule
\end{tabular}
\end{table}

\begin{table*}[t]\small
\centering
\vspace{-2ex}
\caption{Few-shot classification results. We report mean and std over 10 runs. We bold the the cell with the largest mean. We also bold the cell where its mean + std $>=$ the largest mean.}
\begin{tabular}{l|cccccccc}
\bottomrule \multicolumn{1}{c|}{\multirow{3}{*}{Baseline}} & 
\multicolumn{4}{c}{ModelNet40} & \multicolumn{4}{c}{Sydney10} \\ \cline{2-9}
& \multicolumn{2}{c}{5-way} & \multicolumn{2}{c}{10-way} & \multicolumn{2}{c}{5-way} & \multicolumn{2}{c}{10-way}\\ \cline{2-9}
& 10-shot & 20-shot & 10-shot & 20-shot & 10-shot & 20-shot & 10-shot & 20-shot \\ \toprule \bottomrule
3D-GAN, Rand & 55.8$\pm$10.7 & 65.8$\pm$9.9 &40.3$\pm$6.5 &48.4$\pm$5.6 & 54.2$\pm$4.6 & 58.8$\pm$5.8 & 36.0$\pm$6.2 & 45.3$\pm$7.9\\
FoldingNet, Rand & 33.4 $\pm$13.1 & 35.8$\pm$18.2 & 18.6$\pm$6.5 & 15.4$\pm$6.8 & 58.9$\pm$5.6 & 71.2$\pm$6.0 & 42.6$\pm$3.4 & 63.5$\pm$3.9\\
Latent-GAN, Rand & 41.6$\pm$16.9 & 46.2$\pm$19.7 & 32.9$\pm$9.2 & 25.5$\pm$9.9 & 64.5$\pm$6.6 & 79.8$\pm$3.4 & 50.5$\pm$3.0 & 62.5$\pm$5.1\\
PointCapsNet, Rand & 42.3$\pm$17.4 &53.0$\pm$18.7 &38.0$\pm$14.3 & 27.2$\pm$14.9 & 59.4$\pm$6.3 & 70.5$\pm$4.8 & 44.1$\pm$2.0 & 60.3$\pm$4.9\\
PointNet++, Rand & 38.5$\pm$16.0 & 42.4$\pm$14.2 & 23.1$\pm$7.0 & 18.8$\pm$5.4 & \textbf{79.9$\pm$6.8} & {85.0$\pm$5.3} & 55.4$\pm$2.2 & 63.4$\pm$2.8\\
PointCNN, Rand & {65.4$\pm$8.9} & {68.6$\pm$7.0} & {46.6$\pm$4.8} & {50.0$\pm$7.2} & 75.8$\pm$7.7 & 83.4$\pm$4.4 & 56.3$\pm$2.4 & {73.1$\pm$4.1}\\
\toprule \bottomrule
PointNet, Rand & 52.0$\pm$12.2 & 57.8$\pm$15.5 & 46.6$\pm$13.5 & 35.2$\pm$15.3 & 74.2$\pm$7.3 & 82.2$\pm$5.1 & 51.4$\pm$1.3 & 58.3$\pm$2.6\\
% PointNet, Jigsaw & & & & & & & &  \\
PointNet, cTree & 63.2$\pm$10.7 & 68.9$\pm$9.4 & 49.2$\pm$6.1 & 50.1$\pm$5.0 &  76.5$\pm$6.3 & 83.7$\pm$4.0 & 55.5$\pm$2.3 & 64.0$\pm$2.4\\
PointNet, OcCo & \textbf{89.7$\pm$6.1} & \textbf{92.4$\pm$4.9} & \textbf{83.9$\pm$5.6} & \textbf{89.7$\pm$4.6} & {77.7$\pm$8.0} & {84.9$\pm$4.9} & {60.9$\pm$3.7} & {65.5$\pm$5.5}\\\hline
DGCNN, Rand & 31.6 $\pm$9.0 & 40.8$\pm$14.6 &19.9$\pm$6.5 & 16.9$\pm$4.8 & 58.3$\pm$6.6 & 76.7$\pm$7.5 & 48.1$\pm$8.2 &76.1$\pm$3.6\\
% DGCNN, Jigsaw & 34.3$\pm$4.1 & 42.2$\pm$11.0 & 26.0$\pm$7.5 & 29.9$\pm$8.2 & 52.5$\pm$6.6 & 79.6$\pm$6.0 & 52.7$\pm$3.3 & 69.1$\pm$2.6\\
DGCNN, cTree & 60.0$\pm$8.9 & 65.7$\pm$8.4 & 48.5$\pm$5.6 & 53.0$\pm$4.1 & \textbf{86.2$\pm$4.4} & \textbf{90.9$\pm$2.5} & \textbf{66.2$\pm$2.8} & \textbf{81.5$\pm$2.3}\\
DGCNN, OcCo & \textbf{90.6$\pm$2.8} & \textbf{92.5$\pm$6.0} & \textbf{82.9$\pm$4.1} & \textbf{86.5$\pm$7.1} & \textbf{79.9$\pm$6.7} & \textbf{86.4$\pm$4.7} & 63.3$\pm$2.7 & \textbf{77.6$\pm$3.9}\\
\toprule
\end{tabular}
% s}
\vspace{-3ex}
\end{table*}

\newpage
\section{Networks and Training Settings of PCN Encoder}
We sketch the network structures of PCN encoder and output layers for downstream tasks in Figure~\ref{fig:pppcn}.
\begin{figure}[H]
    \centering
     \includegraphics[width=\textwidth]{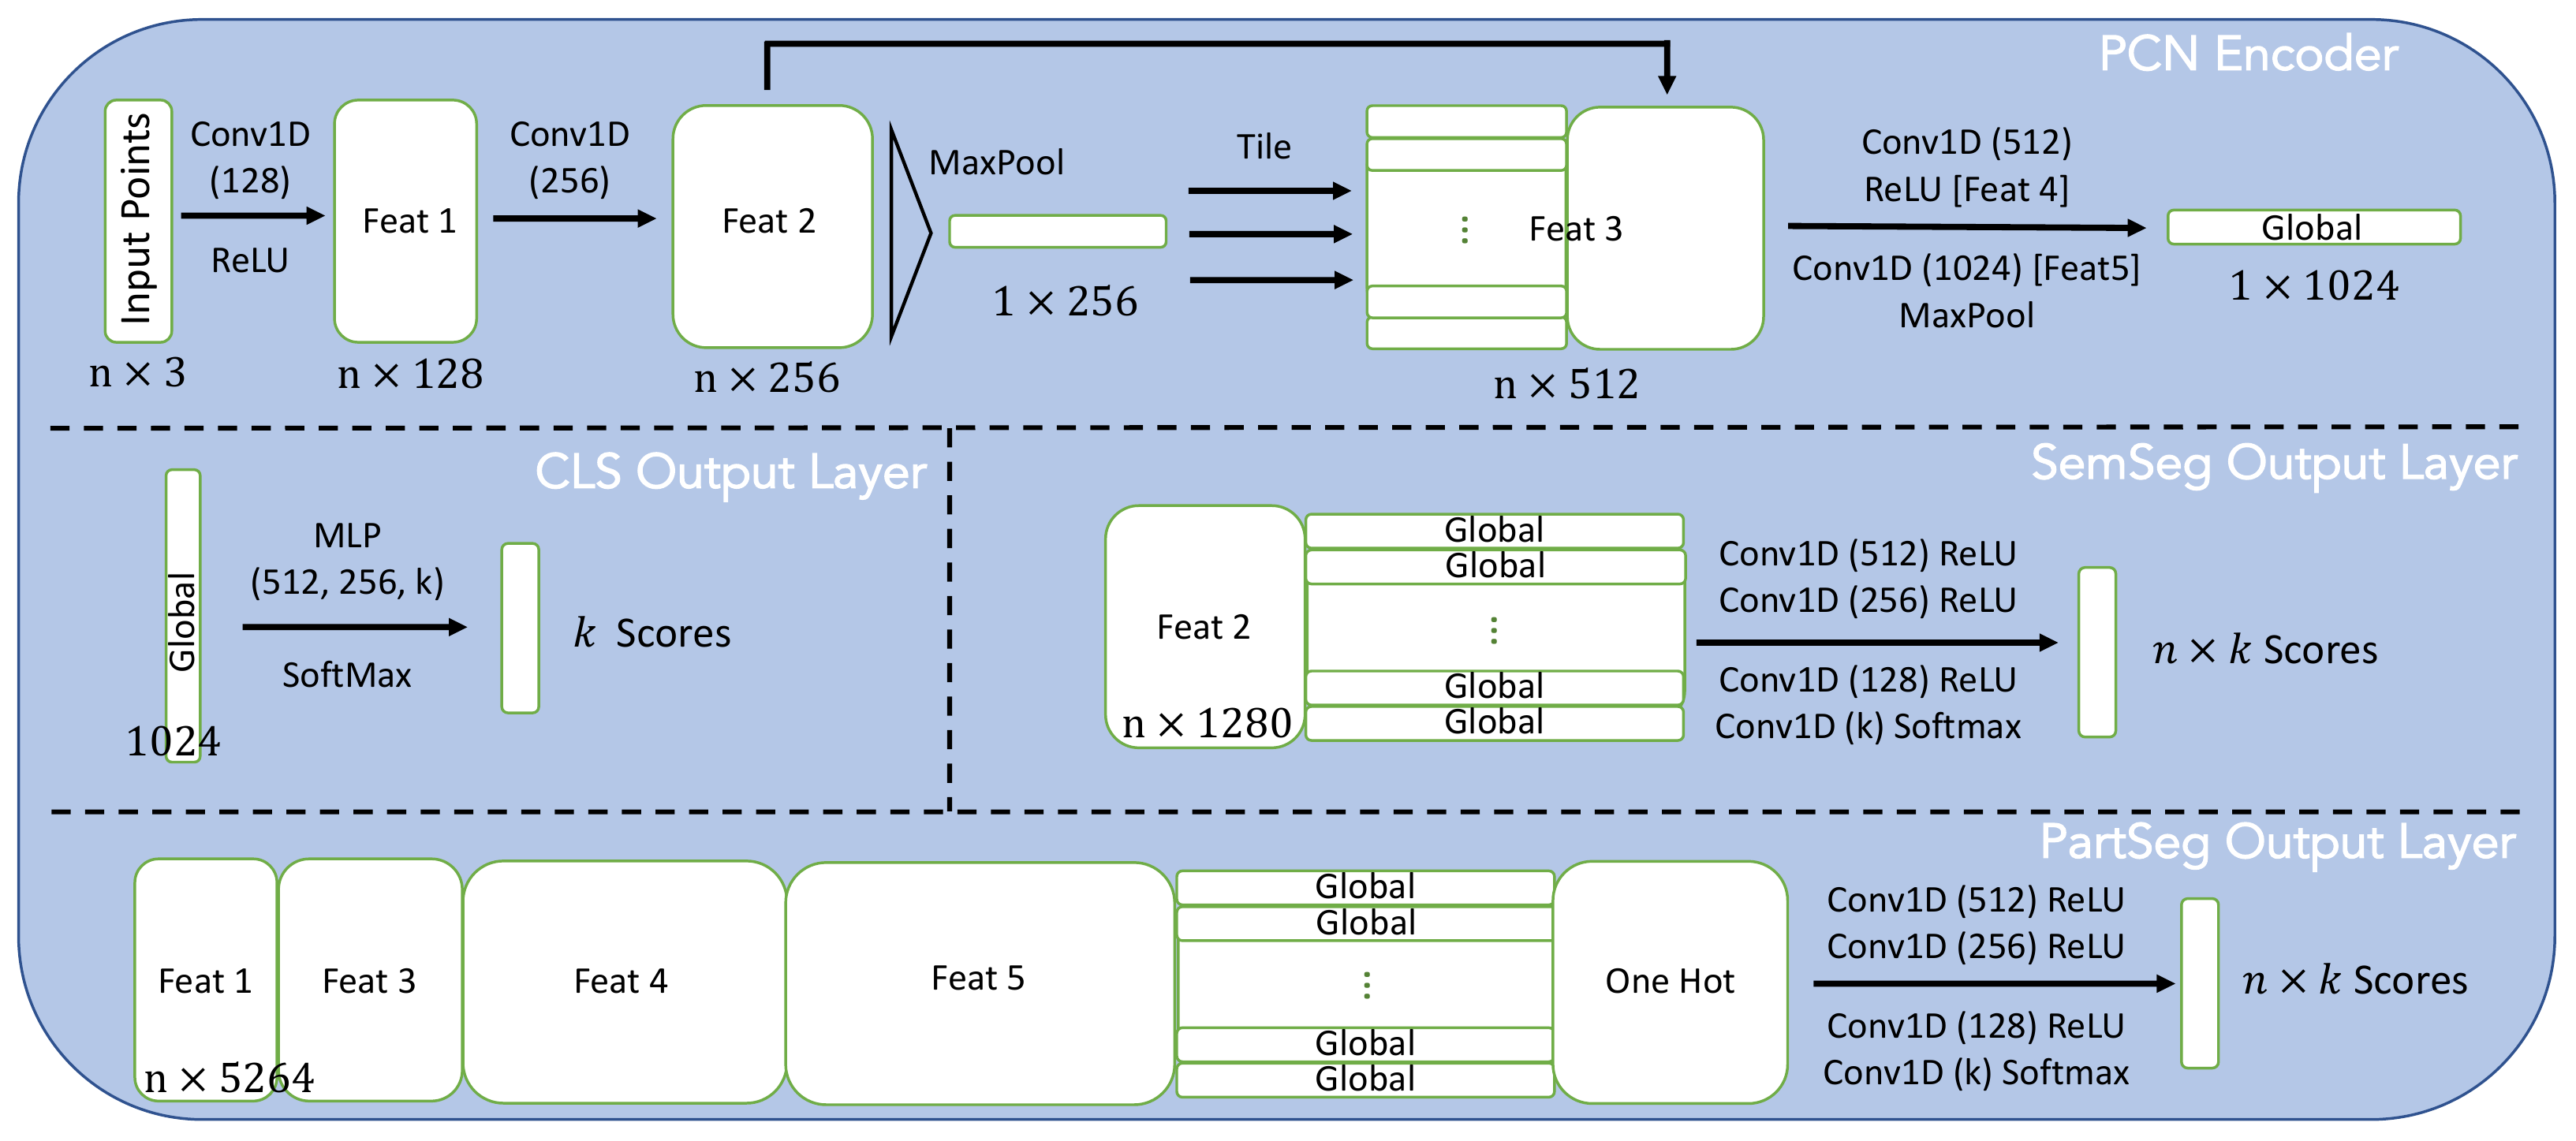}
     \caption{Encoder and Output Layers of PCN}
     \label{fig:pppcn}
\end{figure}

\section{Detailed results of the part segmentation}
Here in Table~\ref{tab:partseg} we report the detailed scores on each individual shape category from ShapeNetPart, we bold the best scores for each class respectively. We show that for all three encoders, OcCo-initialisation has achieved better results over two thirds of these 15 object classes.
\begin{table}[H]
\small
\centering
\caption{Detailed Results on Part Segmentation Task on ShapeNetPart}
\begin{tabular}{c|c|c|c|c|c|c|c|c|c}
\bottomrule \multirow{2}{*}{Shapes} 
& \multicolumn{3}{c|}{PointNet} 
& \multicolumn{3}{c|}{PCN} 
& \multicolumn{3}{c}{DGCNN} \\ \cline{2-10}
 & Rand* & Jigsaw & \abbrev& Rand & Jigsaw & \abbrev & Rand* & Jigsaw* & \abbrev \\ \toprule \bottomrule
% mean (class)&  &  &  & 78.8 & 77.6 &  &  &  & \\\hline
mean (point)& 83.7 & 83.8 & 84.4 & 82.8 & 82.8 & 83.7 & 85.1 & 85.3 & \textbf{85.5} \\\hline
Aero        & 83.4 & 83.0 & 82.9 & 81.5 & 82.1 & 82.4 & 84.2 & 84.1 & \textbf{84.4}\\\hline
Bag         & 78.7 & 79.5 & 77.2 & 72.3 & 74.2 & 79.4 & 83.7 & \textbf{84.0} & 77.5\\\hline
Cap         & 82.5 & 82.4 & 81.7 & 85.5 & 67.8 & \textbf{86.3} & 84.4 & 85.8 & 83.4\\\hline
Car         & 74.9 & 76.2 & 75.6 & 71.8 & 71.3 & 73.9 & 77.1 & 77.0 & \textbf{77.9}\\\hline
Chair       & 89.6 & 90.0 & 90.0 & 88.6 & 88.6 & 90.0 & 90.9 & 90.9 & \textbf{91.0}\\\hline
Earphone    & 73.0 & 69.7 & 74.8 & 69.2 & 69.1 & 68.8 & 78.5 & \textbf{80.0} & 75.2\\\hline
Guitar      & 91.5 & 91.1 & 90.7 & 90.0 & 89.9 & 90.7 & 91.5 & 91.5 & \textbf{91.6}\\\hline
Knife       & 85.9 & 86.3 & 88.0 & 84.0 & 83.8 & 85.9 & 87.3 & 87.0 & \textbf{88.2}\\\hline
Lamp        & 80.8 & 80.7 & 81.3 & 78.5 & 78.8 & 80.4 & 82.9 & 83.2 & \textbf{83.5}\\\hline
Laptop      & 95.3 & 95.3 & 95.4 & 95.3 & 95.1 & 95.6 & 96.0 & 95.8 & \textbf{96.1}\\\hline
Motor       & 65.2 & 63.7 & 65.7 & 64.1 & 64.7 & 64.2 & 67.8 & \textbf{71.6} & 65.5\\\hline
Mug         & 93.0 & 92.3 & 91.6 & 90.3 & 90.8 & 92.6 & 93.3 & 94.0 & \textbf{94.4}\\\hline
Pistol      & 81.2 & 80.8 & 81.0 & 81.0 & 81.5 & 81.5 & \textbf{82.6} & \textbf{82.6} & 79.6\\\hline
Rocket      & 57.9 & 56.9 & 58.2 & 51.8 & 51.4 & 53.8 & 59.7 & \textbf{60.0} & 58.0\\\hline
Skateboard  & 72.8 & 75.9 & 74.2 & 72.5 & 71.0 & 73.2 & 75.5 & \textbf{77.9} & 76.2 \\\hline
Table       & 80.6 & 80.8 & 81.8 & 81.4 & 81.2 & 81.2 & 82.0 & 81.8 & \textbf{82.8} \\\hline
\end{tabular}
\label{tab:partseg}
\vspace{-1ex}
\end{table}

\newpage
\section{Algorithmic Description of OcCo}
\begin{lrbox}{\codebox}
\begin{lstlisting}
# P: an initial point cloud
# K: camera intrinsic matrix
# V: number of total view points
# loss: a loss function between point clouds
# c: encoder-decoder completion model
# p: downstream prediction model

while i < V:
    # sample a random view-point
    R_t = [random.rotation(), random.translation()]
    
    # map point cloud to camera reference frame
    P_cam = dot(K, dot(R_t, P))
    
    # create occluded point cloud
    P_cam_oc = occlude(P_cam, alg='z-buffering')
    
    # point cloud back to world frame
    K_inv   = [inv(K), zeros(3,1); zeros(1,3), 1]
    R_t_inv = transpose([R_t; zeros(3,1), 1])
    P_oc = dot(R_t_inv, dot(K_inv, P_cam_oc))

    # complete point cloud
    P_c = c.decoder(c.encoder(P_oc))
    
    # compute loss, update via gradient descent
    l = loss(P_c, P)
    l.backward()
    update(c.params)
    i += 1

# downstream tasks, use pre-trained encoders
p.initialize(c.encoder.params)
p.train()
\end{lstlisting}
\end{lrbox}

\begin{algorithm}[H]
  \caption{Occlusion Completion (OcCo)}\label{alg:occo}
  \usebox{\codebox}
\end{algorithm}

\newpage
\noindent\begin{figure}[H]
    \centering
    \includegraphics[width=\textwidth]{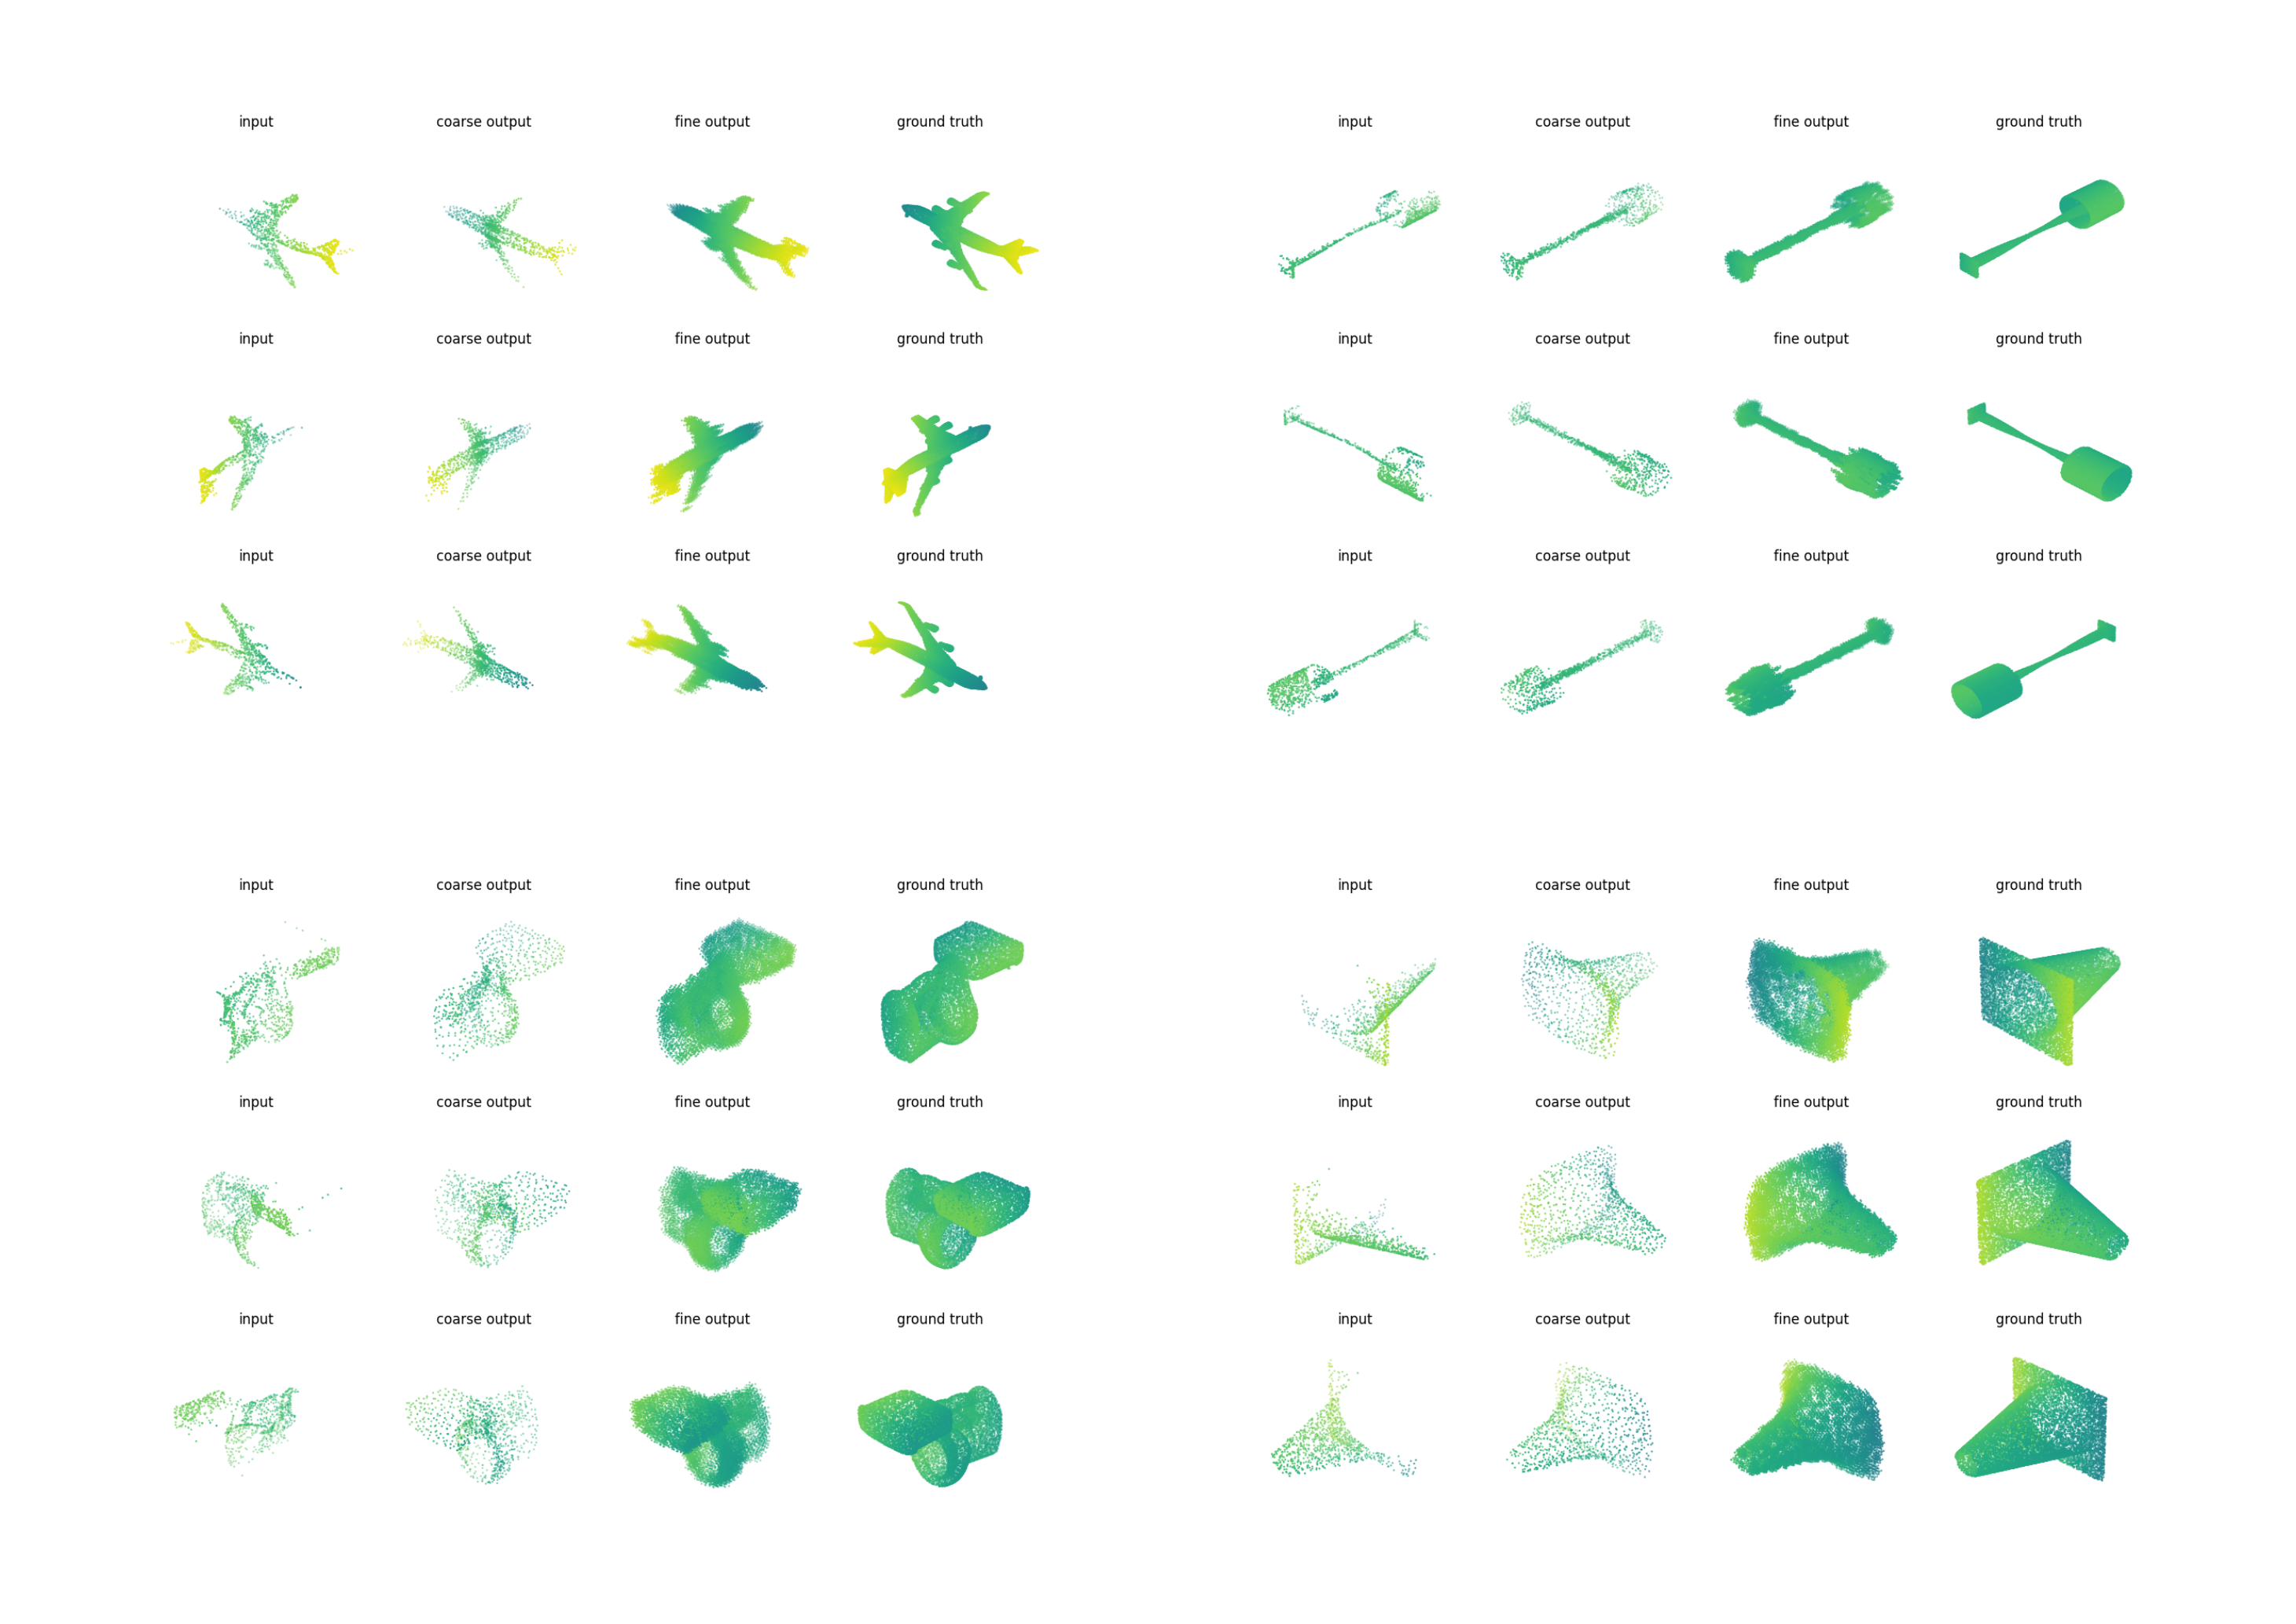}
    \caption{OcCo pre-training with PCN encoder on occluded ModelNet40.}
    \label{fig:qualitative_occo_pcn}
\end{figure}
\newpage
\noindent\begin{figure}[H]
    \centering
    \includegraphics[width=\textwidth]{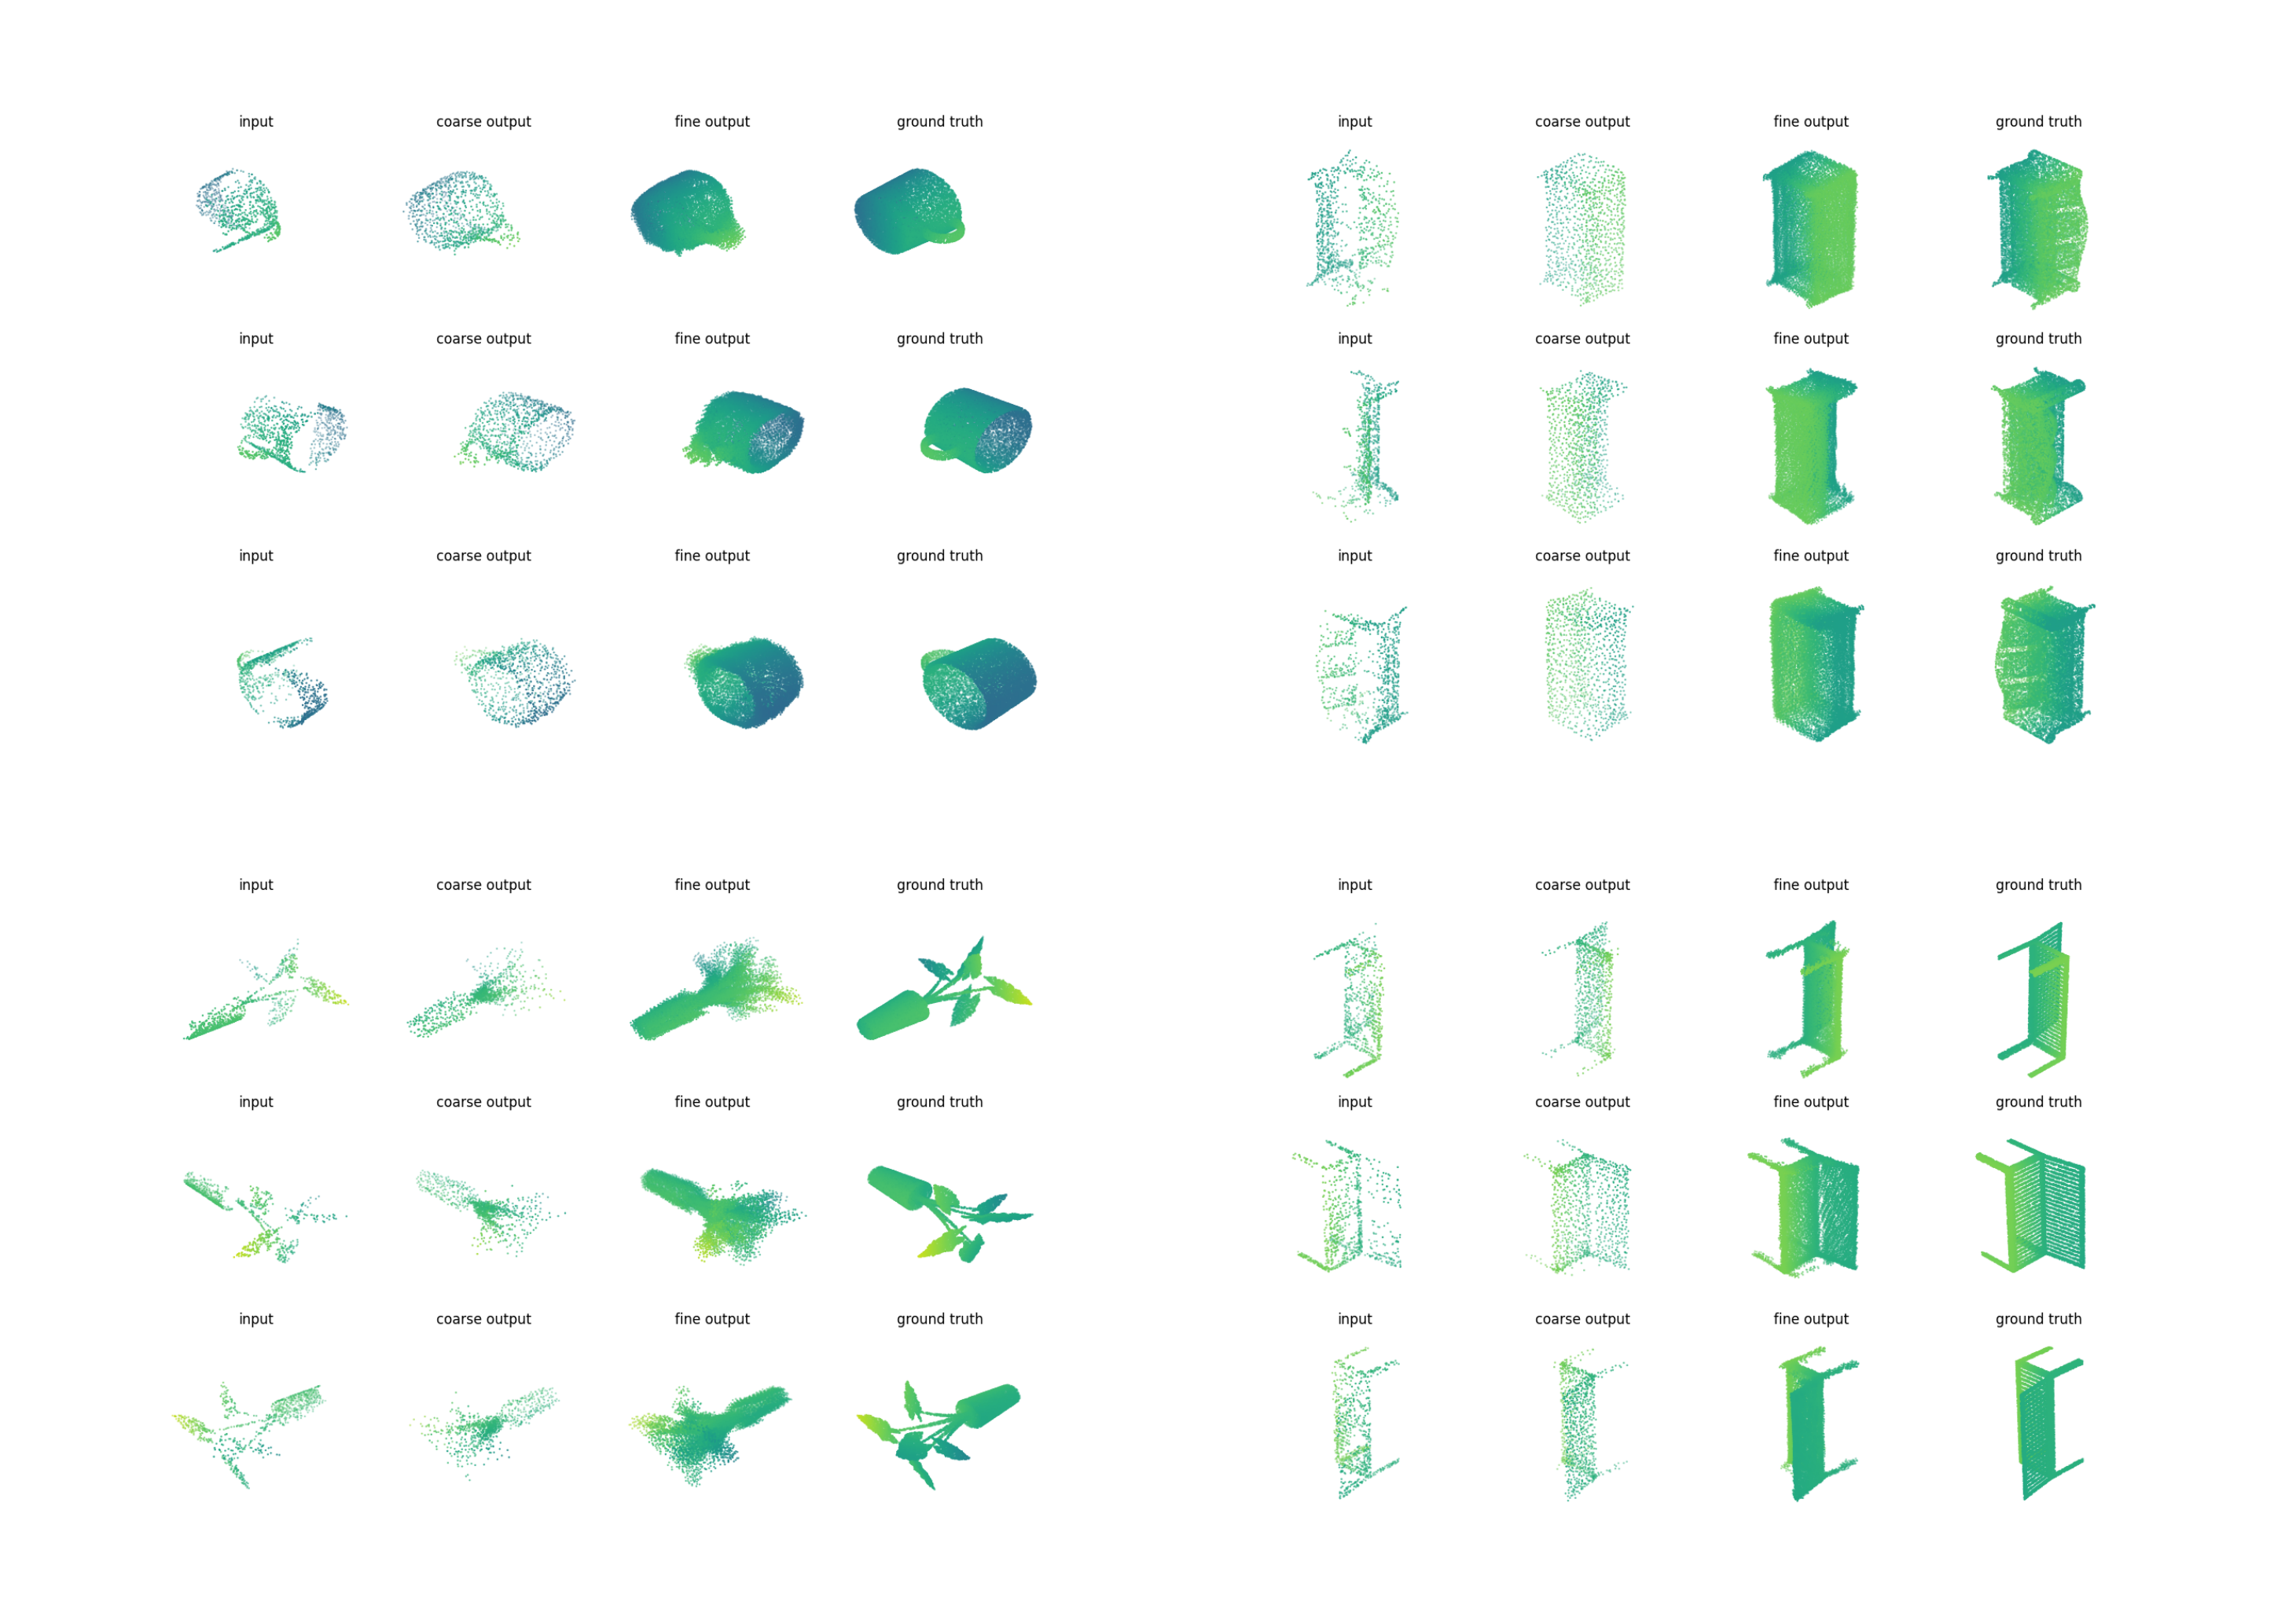}
    \caption{OcCo pre-training with PointNet encoder on occluded ModelNet40.}
    \label{fig:qualitative_occo_pointnet}
\end{figure}
\newpage
\noindent\begin{figure}[H]
    \centering
    \includegraphics[width=\textwidth]{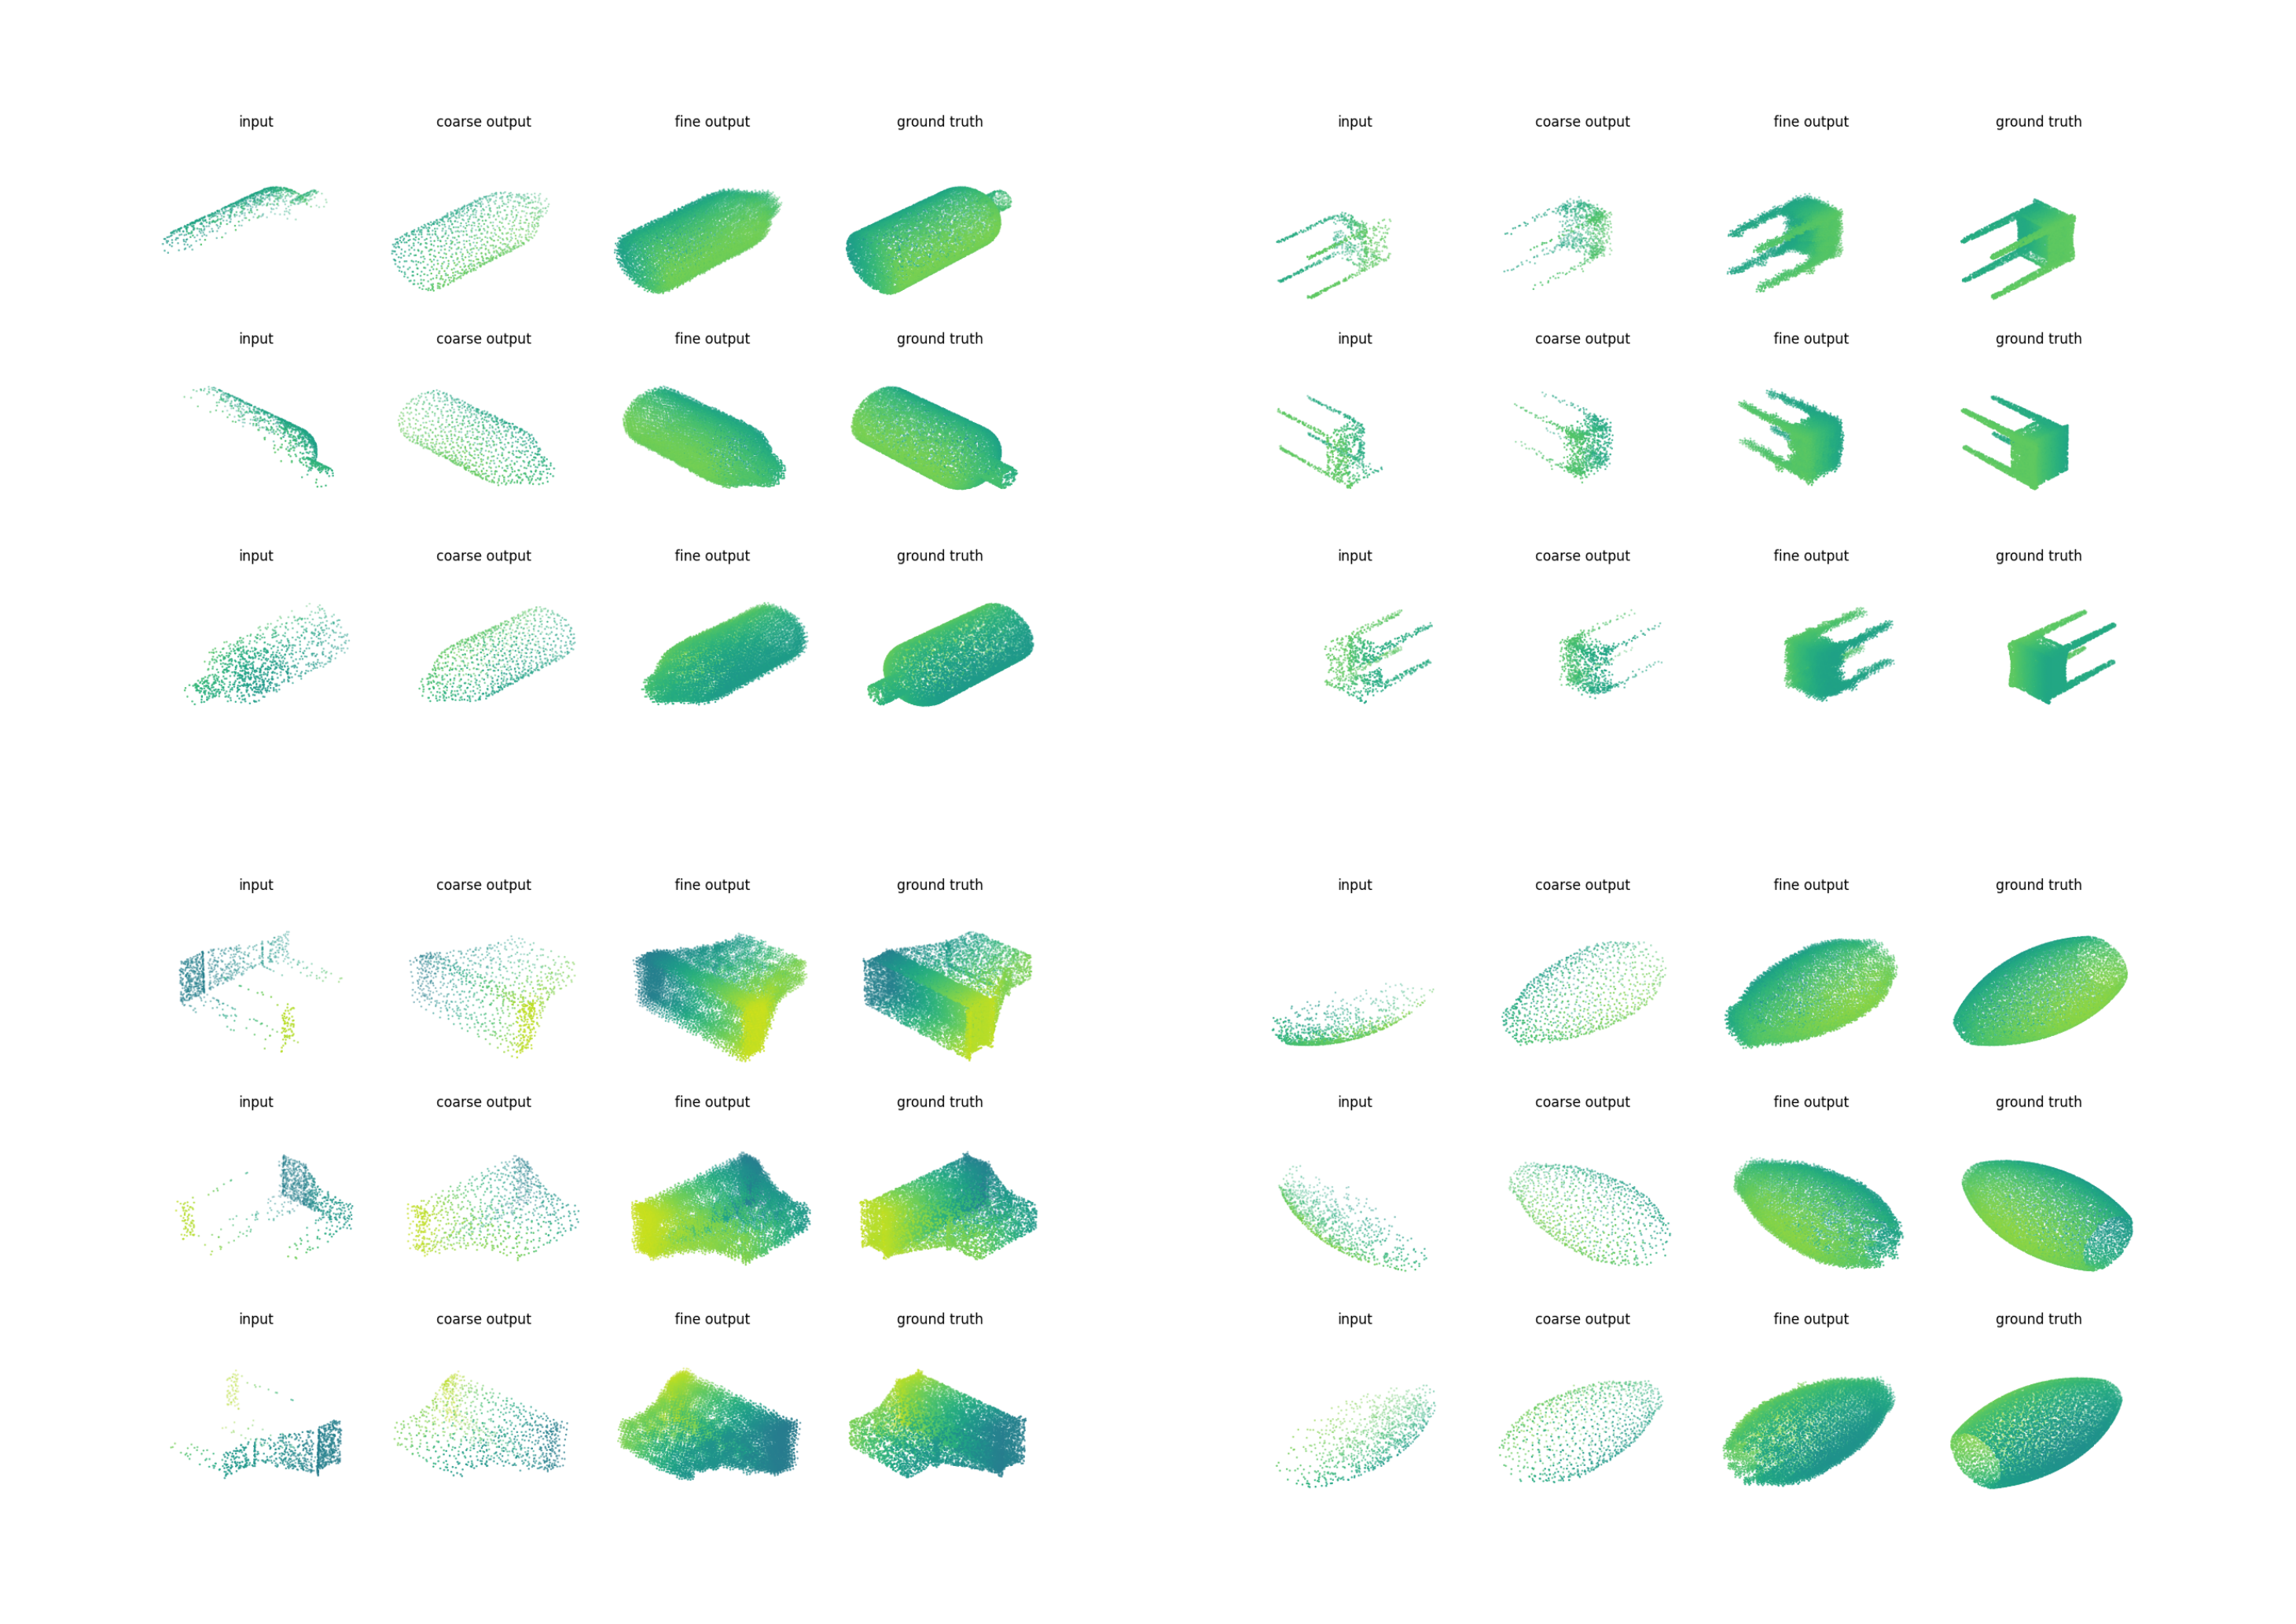}
    \caption{OcCo pre-training with DGCNN encoder on occluded ModelNet40.}
    \label{fig:qualitative_occo_dgcnn}
\end{figure}
% However we also observe that the completion models have difficulties at completing complex shapes e.g., hollow structures. We think this is probably because the folding-based generator/decoder are good at generating smooth surfaces, which might not be suitable for things such as handrails.
\begin{figure}[H]
    \centering
     \includegraphics[width=\textwidth]{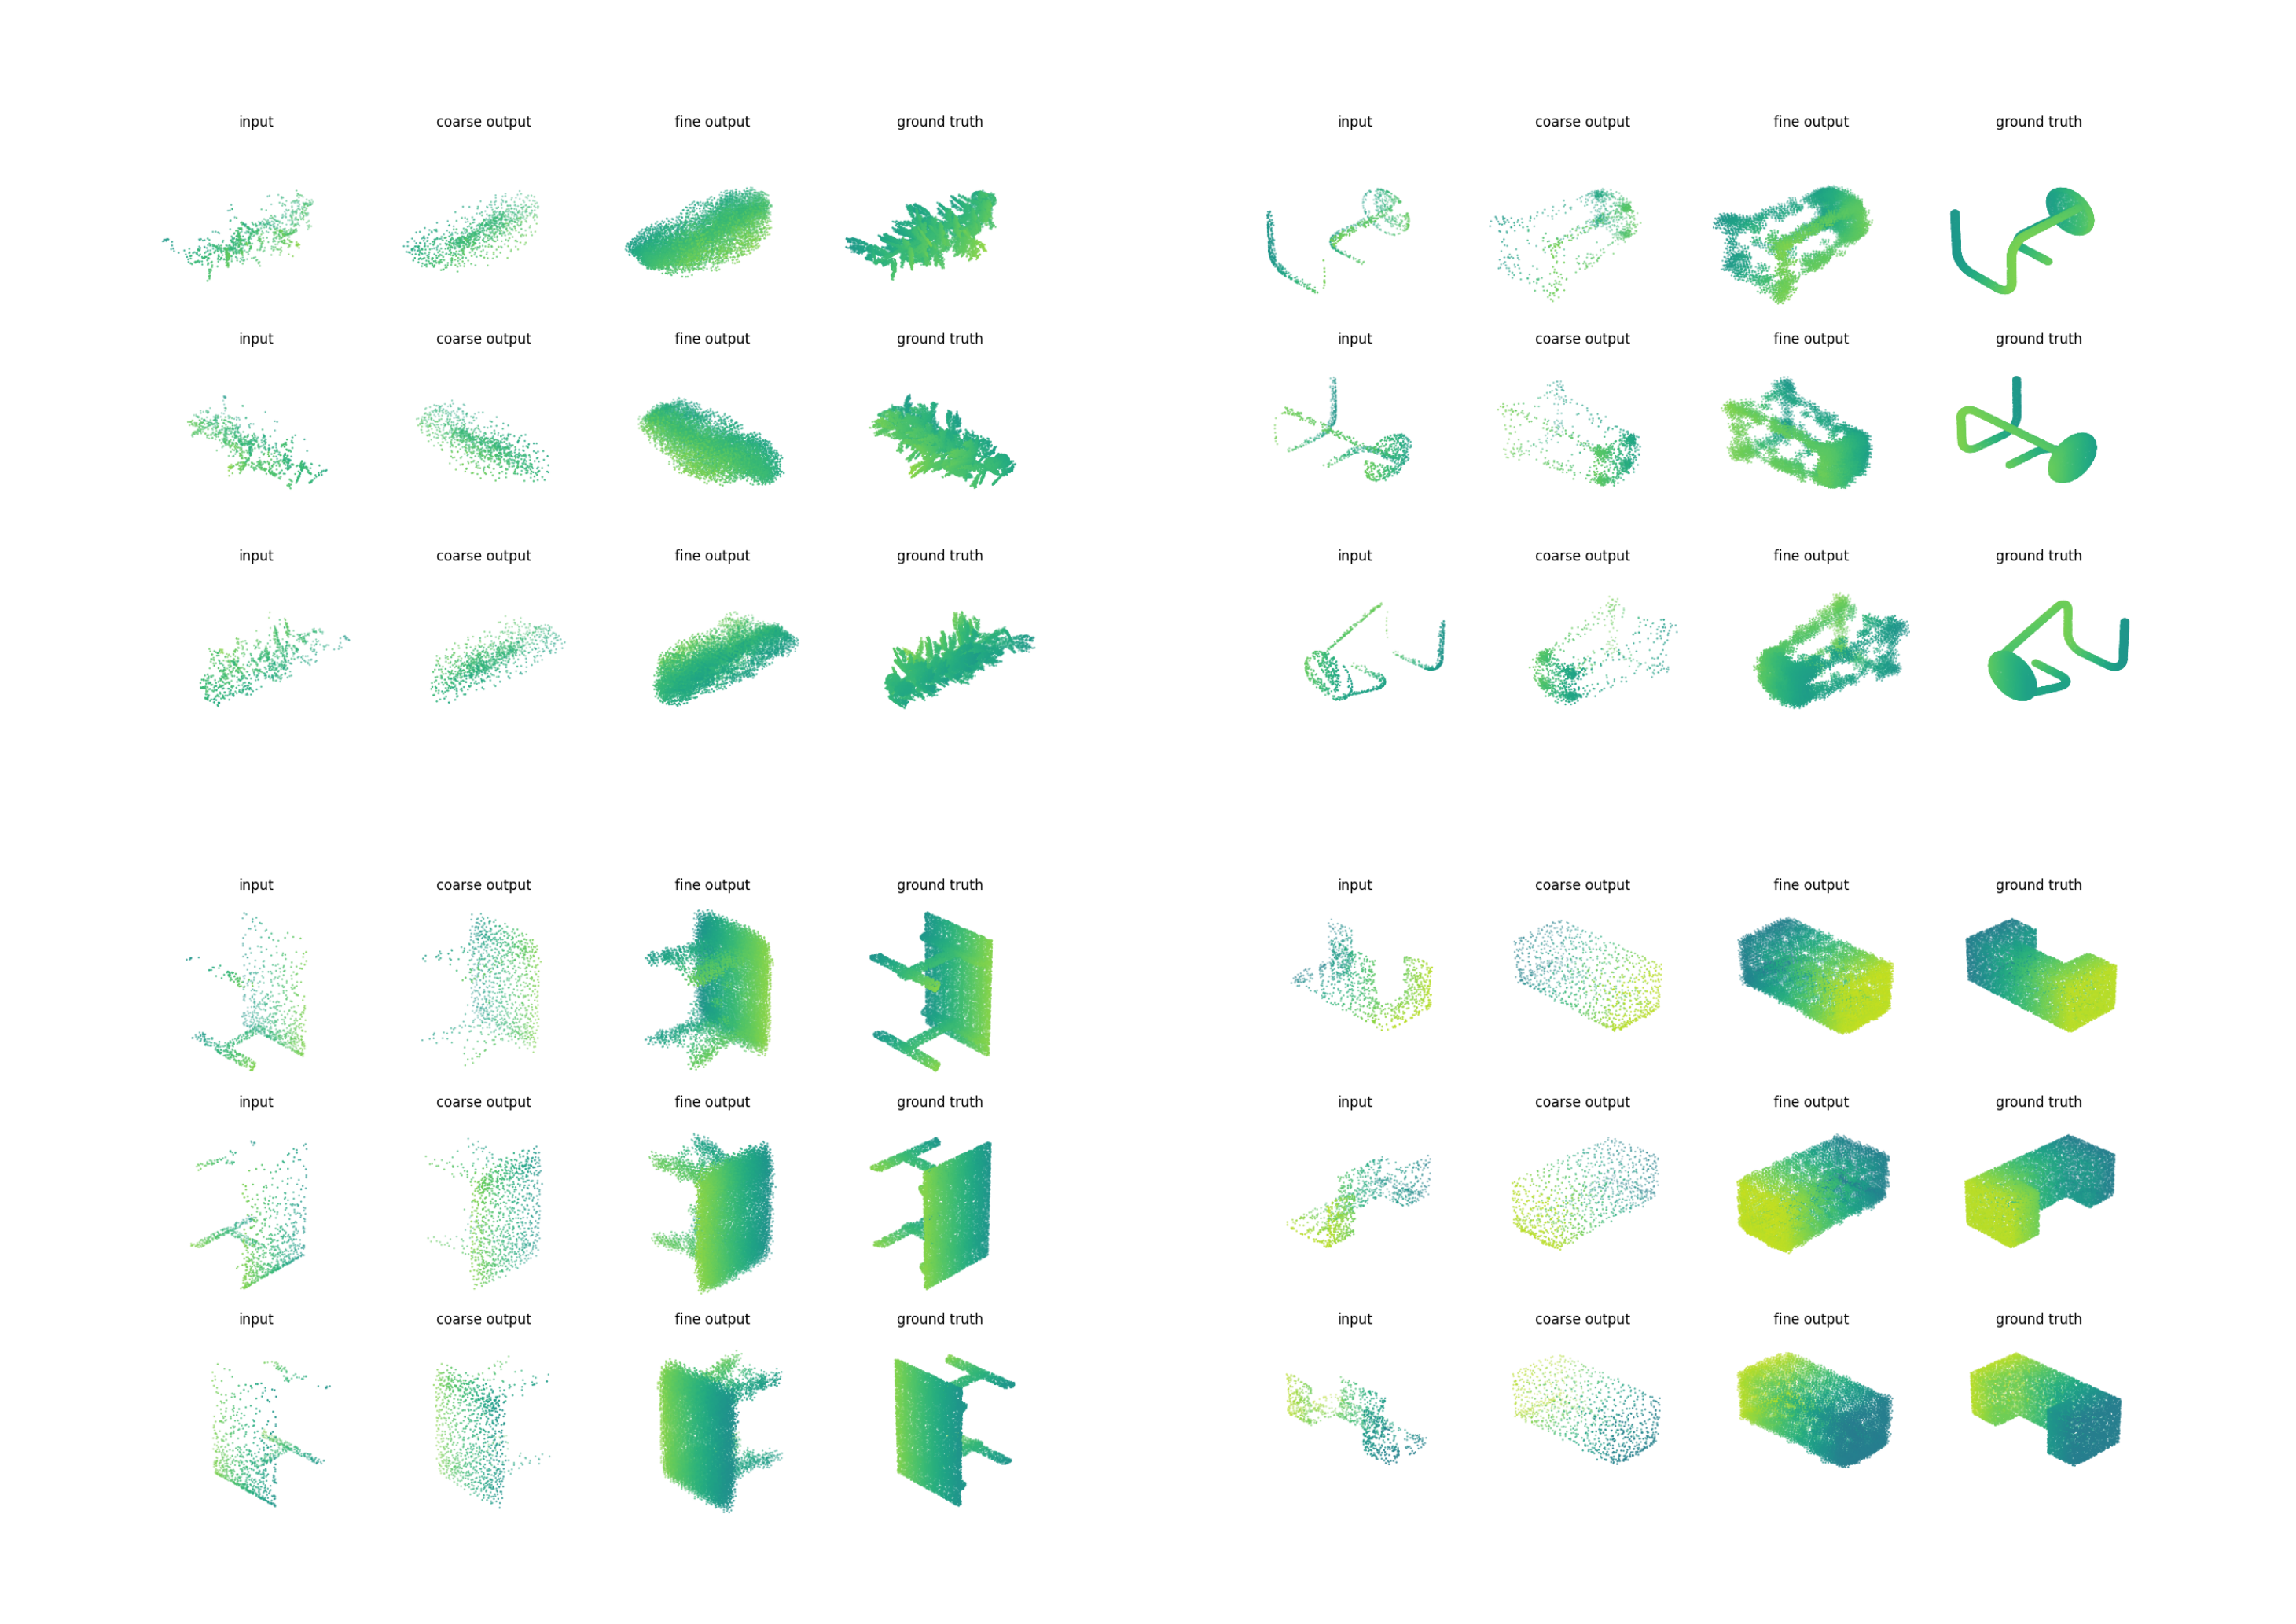}
     \caption{Failure completed examples during OcCo pre-training.}
     \label{fig:failuare_occo}
\end{figure}
